# Supplementary material for: On the Dynamics of Liquids in the Large-Dimensional Limit
Source: arXiv:2108.02378 ancillary file (2021-08-05)
Supplement: Supplementary file 1 [file SI.pdf]

# Supplemental Information

Chen Liu
*Laboratoire de Physique de l'Ecole normale supérieure, ENS, Université PSL, CNRS, Sorbonne Université, Université de Paris, F-75005 Paris, France and Department of Chemistry, Columbia University, New York, New York 10027, USA*

Giulio Biroli
*Laboratoire de Physique de l'Ecole normale supérieure, ENS, Université PSL, CNRS, Sorbonne Université, Université de Paris, F-75005 Paris, France*

David R. Reichman
*Department of Chemistry, Columbia University, New York, New York 10027, USA*

Grzegorz Szamel
*Department of Chemistry, Colorado State University, Fort Collins, CO 80525, USA*

This supplemental material provides all supporting information to our main text and details of computations of our three methods. Sec.I – III discuss general aspect of dimensional scales of dynamic variables in the $d \to \infty$ mean-field limit, as well as various simplifications implied purely by geometry, which serve Sec.VI to justify that the memory kernels for one and two particle processes are identical. Sec.IV and V detail the computation of the Newtonian case using projection operator formalism. Sec.VII and VIII show the complete computation for the Brownian case using projection operator. Sec.IX – XI present the whole set of cavity method. Sec.X justifies the key passage from Eq.5 to Eq.7 in the main text, which is applicable to all our three approaches. This section presents general arguments and can be read independently. Sec.XII presents the final simplified set of scalar equations that gives way for self-consistent resolution. Sec.XIII derives the random Lorentz gas equations using our method. Sec.XIV sketches our perspective in developing a cluster dynamic mean-field theory (cDMFT). Note also that some notations are repeatedly used across different sections for formally different definitions but in analogy with each other across different methods.

## I. DIMENSIONAL SCALE OF DISPLACEMENT

There is an intuitive way to derive the scaling of the displacement $\boldsymbol{u}$ with the dimension $d$ large. It is established that for the energy of the system to be extensive in large dimensions, the interaction potential needs to satisfy

$$v(r) \propto |r/\ell|^{-d-\delta} \quad \text{with}\, \delta > 0, \tag{1}$$

where $\ell \equiv 1$ sets the interaction range [1]. Assuming that we study the system within a time scale where the interaction potential plays a role for the physics, meaning that $v(r)$ neither diverges nor vanishes, implies that $r$ should be close to 1 and in particular the fluctuation of $\Delta r \hat{=} r - 1$ should satisfy

$$v(1+\Delta r) \propto (1+\Delta r)^{-d-\delta} \sim 1. \tag{2}$$

Discarding the $\delta \sim 1$ in front of $d$, $\Delta r$ should be of order $d^{-1}$ for the above equation to be satisfied. Since $v \sim 1$ as well as $d\Delta r = d(r-1) \sim 1$, a natural variable change leads to

$$v(r) \equiv \bar{v}(d(r/\ell - 1)), \tag{3}$$

as mentioned in the main text.

If $\boldsymbol{r}(t) = \boldsymbol{r}(0) + \boldsymbol{u}(t)$, where $r(0) = |\boldsymbol{r}(0)| \sim 1$ and $\boldsymbol{u} = \boldsymbol{u}_0 - \boldsymbol{u}_1$ is the relative displacement between two interacting particles, labeled "0" and "1", then we have, up to the first order in the Taylor expansion,

$$r(t) \approx r(0) + \hat{\boldsymbol{r}}(0)\cdot \boldsymbol{u}(t) + \frac{\boldsymbol{u}^2}{2r(0)}. \tag{4}$$

We deduce $\hat{\boldsymbol{r}}(0)\cdot\boldsymbol{u} + \boldsymbol{u}^2 \sim \Delta r \sim d^{-1}$, where $\hat{\boldsymbol{r}}(0)\cdot\boldsymbol{u}$ can be viewed as an arbitrary component of $\boldsymbol{u}$. This implies $u_\mu \sim u_{0,\mu} \sim u_{1,\mu} \sim d^{-1}$ for arbitrary component $\mu$ and $\boldsymbol{u}^2 = \sum_{\mu=1}^d u_\mu^2 \sim d(d^{-1})^2 \sim d^{-1}$. Note that $u_\mu$ is fluctuating in amplitude of order $d^{-1}$ around 0, while $\boldsymbol{u}^2$ has a positive value of order $d^{-1}$. Actually we have $\boldsymbol{u}^2 = \boldsymbol{u}_1^2 + \boldsymbol{u}_2^2 - 2\boldsymbol{u}_1\cdot\boldsymbol{u}_2$. The cross product is sub-leading as $2\sum_{\mu=1}^d u_{0,\mu}u_{1,\mu} \sim d^{1/2}d^{-1}d^{-1} \sim d^{-3/2}$, where the summation $\sum_{\mu=1}^d$ contributes an order $d^{1/2}$ since it runs over terms alternating in sign. The square term e.g. $\boldsymbol{u}_0^2 = \sum_{\mu=1}^d u_{0,\mu}^2$ sums up $d$ positive terms of order $d^{-2}$, thus gives a positive value of order $d^{-1}$. The fluctuation of $\boldsymbol{u}_0^2$ can be estimated using central limit theorem as $\sqrt{d(\langle u_{0,\mu}^4\rangle - \langle u_{0,\mu}^2\rangle^2)} \sim \sqrt{dd^{-4}} \sim d^{-3/2}$, thus sub-leading. That is $\Delta_u$ and $\Delta_w$ (defined in the main text) concentrate on the its average as twice of the mean-square displacement.

In Eq.2 of the main text, the dimensional scaling of the summation of the forces due to effectively interacting particles (i.e. nearest neighboring particles see Sec.II)

along an arbitrary component is estimated based on $v' = d\bar{v}' \sim d$ and $\sum_{\mu=1}^{d} \hat{R}_\mu^2 = 1 \implies \hat{R}_\mu \sim d^{-1/2}$:

$$\sum_{j(\neq i)}^{\sim d} \nabla_\alpha v = \sum_{j(\neq i)}^{\sim d} \hat{R}_{ij,\alpha} v' \sim d^{1/2} d^{-1/2} d \sim d. \tag{5}$$

where we assumed in a large $d$ dimensional space, the number of nearest neighbor is order $\mathcal{O}(d)$ and the summation $\sum_{j(\neq i)}^{\sim d}$ contributes an order of $d^{1/2}$ as the summed terms alternates in sign. All other scaling relations such as $\zeta \sim m \sim d^2$ (which implies $\xi_\mu \sim d$) are natural for balancing the exact dynamic equations Eq.1 of the main text.

## II. GENERAL CONSIDERATIONS OF THE DYNAMICS IN $d \to \infty$ LIMIT

In this section, we justify, from a geometric point of view, that the dynamics in the mean-field limit $d \to \infty$ reduces to a canonical form, namely: (i) For each particle, only the interactions with its first neighbors play a role for its dynamics. (ii) The probability that a third particle interacts simultaneously with two particles that are first neighbors to each other is exponentially small in $d$, i.e. there are effectively no loops of interactions, which makes an infinite dimensional system behave as the Mari-Krzakala-Kurchan model [2].

According to the infinite dimensional potential Eq.1, the force received from a particle lying in the second coordination shell is $\mathcal{O}(2^{-d})$ times smaller than from a first neighbor particle. Knowing that the force along an arbitrary component $\hat{\boldsymbol{e}}_\alpha$ due to a particle of the nearest neighbors is order $\hat{r}_\alpha v' \sim d^{-1/2} d \sim d^{1/2}$, the same component of the force from a second nearest neighbor particle is order $2^{-d} d^{1/2}$. Meanwhile, there are a much larger number of particles in the second coordination shell, as the volume of the second coordination shell is about $2^d$ times larger than the first coordination shell. However when summing up forces coming from all directions, the summation over particles in the second coordination contributes only a order of magnitude $2^{d/2} d^{1/2}$, given that there are $\mathcal{O}(d)$ particles in the first coordination shell. Thus the overall $\alpha$ component of the force coming from the second nearest neighbors is order $2^{d/2} 2^{-d} d \sim 2^{-d/2} d$, which is exponentially smaller in $d$ than the force from the nearest neighbors. As a consequence, each particle effectively interacts only with its nearest neighbors.

To justify the second statement mentioned at the beginning of this section, we consider two particles labelled 0 and 1 lying in the shell of the nearest neighbors of each other, i.e. $|\boldsymbol{R}_0 - \boldsymbol{R}_1| \sim \ell \equiv 1$ . We define a region $I$

$$I \hat{=} \{\boldsymbol{x} | (\boldsymbol{x} - \boldsymbol{R}_0)^2 = (\boldsymbol{x} - \boldsymbol{R}_1)^2 = \ell \equiv 1\}, \tag{6}$$

where particles lie in the shell of the nearest neighbors of both particles 0 and 1, thus interacting with them both. We set $\boldsymbol{R}_0 = \boldsymbol{0}$ and $\boldsymbol{R}_1 = \hat{\boldsymbol{e}}_1$, where $\hat{\boldsymbol{e}}_1$ is one component direction of the Cartesian coordinates. The region $I$ can then be explicitly written as

$$x_1 = 1/2, \quad \sum_{\mu=2}^{d} x_\mu^2 = 3/4, \tag{7}$$

which defines a $d-1$-ball of radius $\sqrt{3}/2$ giving a volume $V_I$ of order $(\sqrt{3}/2)^{d-2} \frac{\pi^{(d-1)/2}}{\Gamma((d-1)/2)}$. Knowing that the first coordination shell is a $d$-ball of radius 1 occupying a volume $V_{1\text{st}}$ of order $\frac{\pi^{d/2}}{\Gamma(d/2)}$, the portion of particles interacting with both particles 0 and 1 among the nearest neighbors of either one is then $V_I / V_{1\text{st}} \sim (\sqrt{3}/2)^d$, which is exponentially small in $d$. Thus the interaction loops of third or higher orders can be neglected in the mean-field theory.

With the above arguments, we derive the following statement. In the mean-field limit, when considering the dynamics of two interacting particles embedded among others, the fluctuating forces and the associated responding friction on each of the two particles are exactly the same as when considering the dynamics of only one particle embedded in the bath of other particles. Because of (i) and (ii), we can assign a tree graph $G(V, E)$ for the effective interactions among particles, using particles as the vertices $V$ and edges $E$ for effective interactions. In this case, the system is expected to behave similarly to the Mari-Krzakala-Kurchan model. This simplification gives way for important implications on the Boltzmann weight on the configuration space of particle positions in the mean-field limit $d \to \infty$ , which we detail in the next section.

## III. BOLTZMANN WEIGHT IN THE LIMIT $d \to \infty$

The true Boltzmann weight on the configuration space of particle positions is formally written

$$e^{-\beta \sum_{i<j} v(\boldsymbol{R}_i - \boldsymbol{R}_j)}. \tag{8}$$

According to Sec.II, the situation such as $v(\boldsymbol{R}_1 - \boldsymbol{R}_2) \sim v(\boldsymbol{R}_2 - \boldsymbol{R}_3) \sim v(\boldsymbol{R}_3 - \boldsymbol{R}_1) \sim \mathcal{O}(1)$, or those that imply higher order loops are intrinsically extremely improbable in the limit $d \to \infty$ for purely geometric reasons. As a consequence, the Boltzmann weight on the entire space can be partitioned into sub-domains, each of them $\mathcal{V}(G)$ being associated with a tree graph $G(V, E)$. A certain tree graph $G(V, E)$ representing effective interactions among particles holds for a configuration $\{\boldsymbol{R}_i\}_i$, if and only if $\{\boldsymbol{R}_i\}_i \in \mathcal{V}(G)$. Each vertex $i \in V$ is labelled by the particle $\boldsymbol{R}_i$. An edge $(i, j) \in E$ states that the two adjacent particles stay in the range of interaction, i.e. $|\boldsymbol{R}_i - \boldsymbol{R}_j| = 1 + h_{ij}/d$, with $|h_{ij}| \sim \mathcal{O}(1)$. A missing edge $(i, k) \notin E$ means the two particles are far apart $|\boldsymbol{R}_i - \boldsymbol{R}_k| \gtrsim 2$. Note that different interaction graphs can be obtained by permuting vertices labels. Thus all subdomains $\mathcal{V}(G)$ for different graphs are statistically equivalent and we only need to study the Boltzmann weight

on a sub-domain $\mathcal{V}(G)$ of a particular graph, for it is representative of that on the entire configuration space.

Let's consider a particular graph $G(V,E)$ where the "central" vertex labelled by particle $\boldsymbol{R}_0$ interacts with $\mathcal{O}(d)$ neighbors including particle $\boldsymbol{R}_1$. The Boltzmann weight on $\mathcal{V}(G)$ then simplifies to

$$\begin{aligned} P_C(\boldsymbol{R}_0,\boldsymbol{R}_1,\ldots)&= \frac{1}{Z_C}e^{-\beta\frac{1}{2}\sum_i\sum_{j\in\partial_i}v(\boldsymbol{R}_i-\boldsymbol{R}_j)} \\ &= \frac{1}{Z_C}e^{-\beta\sum_{(ij)\in E}v(\boldsymbol{R}_i-\boldsymbol{R}_j)}, \\ \text{with } (\boldsymbol{R}_0,\boldsymbol{R}_1,\ldots)&\in\mathcal{V}(G), \end{aligned} \quad (9)$$

where $\partial_i\equiv\{j|(ij)\in E\}$ represents the neighbors of particle $i$ and $Z_C$, the normalization, reads

$$Z_C=\int_{\mathcal{V}(G)}d\boldsymbol{R}_0d\boldsymbol{R}_1d\boldsymbol{R}_2\ldots e^{-\beta\sum_{(ij)\in E}v(\boldsymbol{R}_i-\boldsymbol{R}_j)}. \quad (10)$$

It is then easy to get rid of the couplings between integrated variables by performing the following changes of variables. Firstly, thanks to the tree structure, the vertices can be categorized by "layers" at different graph distances from the "central" vertex particle 0. The $m$-th layer $V_m$ consists of all the vertices to be reached from particle 0 by $m$ edges (the 0-th layer being just particle 0 itself). Hence, $V_m$ contains $d(d-1)^{m-1}\sim d^m$ particles (vertices). Secondly, instead of working with the particles' absolute positions, it is convenient to work with the relative position of a particle of layer $V_m$ with respect to its unique neighbor in layer $V_{m-1}$. For the $m$-th layer we have the relative positions $D_m\equiv\{\boldsymbol{R}_{kl}\hat{=}\boldsymbol{R}_k-\boldsymbol{R}_l, k\in V_m,\ l\in V_{m-1},\ (k,l)\in E\}$ and $D_0\equiv\{\boldsymbol{R}_0\}$.

Yet, the domain of integration $\mathcal{V}(G)$ is still a complex object to be clarified. With the above changes of variables, it is easy to recognize that $\mathcal{V}(G)$ is a subset of $\bar{\mathcal{V}}(G)$ defined as

$$\bar{\mathcal{V}}(G)\hat{=}\{\boldsymbol{R}_0\in\mathbb{R}^d\}\times\prod_{(ij)\in E}\{\boldsymbol{R}_{ij}\in\mathbb{S}_{d-1}\}, \quad (11)$$

where $\mathbb{S}_{d-1}$ represents a volumetric shell of tiny but finite $\mathcal{O}(d^{-1})$ thickness attached to the $(d-1)$-sphere of radius 1 centered at $\mathbf{0}$. Thus the Boltzmann weight in Eq.9 can be expressed

$$\begin{aligned} P_C&= \frac{1}{Z_C}e^{-\beta\left(\sum_{ij\in E}v(\boldsymbol{R}_{ij})+\sum_i\sum_{k<l,\in\partial_i}v(\boldsymbol{R}_{ik}-\boldsymbol{R}_{il})\right)}, \\ Z_C&= \int_{\bar{\mathcal{V}}(G)}d\boldsymbol{R}_0\prod_{(ij)\in E}d\boldsymbol{R}_{ij} \\ &\quad e^{-\beta\left(\sum_{ij\in E}v(\boldsymbol{R}_{ij})+\sum_i\sum_{k<l,\in\partial_i}v(\boldsymbol{R}_{ik}-\boldsymbol{R}_{il})\right)}, \end{aligned} \quad (12)$$

where the first sum contains all effective interactions stated by the graph and the second term prevents particles ($k$ and $l$) neighboring to a common one (particle $i$) from overlapping. However, a pure geometric argument similar to the one of sec.II leads to the conclusion that two particles both sitting in the first coordination shell ($\mathbb{S}_{d-1}$) of a third one have extremely small (exponentially small in $d$) probability to overlap even without interactions between them. Formally one can show, with $\theta(x)$ denoting the Heaviside function

$$\frac{1}{\mathbb{S}_{d-1}^2}\int_{\mathbb{S}_{d-1}^2}d\boldsymbol{R}d\boldsymbol{R}'\theta(1+d^{-1}-|\boldsymbol{R}-\boldsymbol{R}'|)\lesssim(\frac{\sqrt{3}}{2})^d.$$

That is, we can release the domain-constraint $\mathcal{V}(G)$ to $\bar{\mathcal{V}}(G)$ for the Boltzmann weight in Eq.9 and conclude

$$P_C= \frac{1}{Z_C}\prod_{(ij)\in E}e^{-\beta v(R_{ij})},\quad \boldsymbol{R}_{ij}\in\mathbb{S}_{d-1},\ \forall(ij)\in E \quad (13)$$

Thus we not only decouple the integrated variables but also we integrate them independently and freely in $\mathbb{S}_{d-1}$. This effectively simplified Boltzmann weight on the configuration space plays an important intermediate step when investigating the derived force-force correlations using the projection operator formalism in the following sections.

Note that Eq.12 and 13 neglect the boundary condition for a finite system, which is necessary for computing the equation of state by direct integration of the partition function as the thermodynamic limit is taken only after the free energy is obtained for a finite system. For our purpose (in Sec.VI) of discussing the dynamics, these equations help to clarify the fact locally the integration variables $\boldsymbol{R}_{ij}$ can be treated as independent from each other in the large system size limit.

## IV. NEWTONIAN PROJECTION OPERATOR FORMALISM

Here, we follow the approach of Mazur and Oppenheim [3] with a modification of the definition of the projection operator tailored to average over all coordinates save the special tagged particle direction $\alpha$. We define the full and unperturbed Liouvillians explicitly as

$$iL=\frac{p_{0,\alpha}}{m}\nabla_{0,\alpha}+F_{0,\alpha}\nabla_{p_{0,\alpha}}+iL_0, \quad (14)$$

where

$$\begin{aligned} iL_0&= \sum_{j>0}\nabla_{\mathbf{p}_j}H_0\cdot\nabla_{\mathbf{R}_j}-\sum_{j>0}\nabla_{\mathbf{R}_j}H_0\cdot\nabla_{\mathbf{p}_j} \\ &\quad+\sum_{\nu\neq\alpha}\left[\frac{p_{0,\nu}}{m}\nabla_{0,\nu}+F_{0,\nu}\nabla_{0,\nu}\right], \end{aligned} \quad (15)$$

$H_0 = \sum_{\nu\neq\alpha}\frac{m}{2}\dot{u}_{0,\nu}^2 + \sum_{j>0}\sum_{\nu=1}^d\frac{m}{2}\dot{u}_{j,\nu}^2 + \sum_{i>j>0}v(\mathbf{R}_{ij}) + \sum_{j>0}v(\mathbf{R}_{0j})$, and $F_{0,\nu}$ is the $\nu^{th}$ component of the force on the tagged particle. The projection operator is defined as

$$\begin{aligned} \mathcal{P}A&= \frac{1}{Z_0}\int d\boldsymbol{R}_{0,\alpha}^{\perp}d\mathbf{p}_{0,\alpha}^{\perp}\prod_{i=1}^N d\mathbf{R}_i\prod_{i=1}^N d\mathbf{p}_iA\exp(-\beta H_0) \\ &= \langle A\rangle_0, \end{aligned} \quad (16)$$

where $d\mathbf{p}_{0,\alpha}^{\perp} = \prod_{\nu\neq\alpha} dp_{0,\nu}$, $Z_0 = \int \prod_{i=1}^{N} d\mathbf{R}_i \prod_{i=1}^{N} d\mathbf{p}_i d\boldsymbol{R}_{0,\alpha}^{\perp} d\mathbf{p}_{0,\alpha}^{\perp} \exp(-\beta H_0)$. Using the exact operator relationship

$$e^{(A+B)t} = e^{At} + \int_0^t e^{A(t-\tau)} B e^{(A+B)\tau} d\tau, \quad (17)$$

and applying this operator identity to the $\alpha^{th}$ component of the tagged particle's force at $t=0$ with the choices $A = iL$ and $B = -i\mathcal{P}L$, we find

$$\dot{p}_{0,\alpha}(t) = F_\alpha^\dagger(t) + \int_0^t d\tau e^{iL(t-\tau)} (\nabla_{p_{0,\alpha}} - \frac{p_{0,\alpha}}{mk_bT}) \langle F_\alpha F_\alpha^\dagger(\tau) \rangle_0, \quad (18)$$

where $F_\alpha^\dagger(t) = e^{i(1-\mathcal{P})Lt} F_{0,\alpha}(0)$ and $F_\alpha \equiv F_\alpha^\dagger(0)$. This is the exact starting point presented in the main text. Note that the Langevin equation derived above is deceptive because it is non-linear and does not have the typical form of a Langevin equation. In particular, the factors $e^{iL(t-\tau)}$ and $\nabla_{p_{0,\alpha}}$ act completely on all terms to the right. Only if the force-force term does not depend on the system variables $u_{0,\alpha}$ and $p_{0,\alpha}$ will the equation result in a standard Langevin form. Below we show how this simplification occurs exactly in the $d \to \infty$ case.

We first show how the fluctuating force simplifies for $d \to \infty$. We expand the the generator of time evolution to lowest non-trivial order as

$$F_\alpha^\dagger(t) \sim (e^{iL_0 t} + \int_0^t d\tau e^{iL_0(t-\tau)} (1-\mathcal{P})(O_P + O_F) e^{iL_0\tau}) F_{0,\alpha}(0) \quad (19)$$

where $O_P = \frac{p_{0,\alpha}}{m} \nabla_{0,\alpha}$ and $O_F = F_{0,\alpha} \nabla_{p_{0,\alpha}}$.

This leads simply to

$$F_\alpha^\dagger(t) \sim \tilde{F}_{0,\alpha}(t) - t \frac{p_{0,\alpha}(0)}{m} (\tilde{k}_\alpha(t) - \langle \tilde{k}_\alpha(t) \rangle_0), \quad (20)$$

where $k_\alpha(0) = \sum_{j>0} \nabla_\alpha \nabla_\alpha v(\boldsymbol{R}_{0j}(0))$ and the notation $\tilde{A}$ denotes that the time dependence occurs with the motion along the $\alpha$ direction blocked, namely it is generated by $L_0$, in particular $\tilde{F}_{0,\alpha}(t) = e^{iL_0 t} F_{0,\alpha}(0)$. Aside from the factor of $t$, the correction to the bare force term scales as $\frac{1}{d} \cdot d^{3/2} \sim d^{1/2}$ (see Sec.IX Eq.87) which is smaller than the $\mathcal{O}(d)$ bare force by a factor of $d^{1/2}$. It is not difficult to show that it is true that the expansion leads, order by order, to terms that are smaller than the leading term in $d$. The secular aspect of the correction term suggests that the limit $d \to \infty$ must be taken before $t \to \infty$.

The expansion of the force-force term is that of a direct Dyson series. In particular

$$\langle F_\alpha F_\alpha^\dagger(t) \rangle_0 = \langle F_{0,\alpha} e^{iL_0 t} F_{0,\alpha} \rangle_0 + I_2 + I_4 + ..., \quad (21)$$

where

$$I_2 = \int_0^t d\tau_1 \int_0^{\tau_1} d\tau_2 G_2(t, \tau_1, \tau_2), \quad (22)$$

$$G_2(t,\tau_1,\tau_2) = \langle F_{0,\alpha} e^{iL_0(t-\tau_1)} (1-\mathcal{P})(O_P + O_F) e^{iL_0(\tau_1-\tau_2)} \times (1-\mathcal{P})(O_P + O_F) e^{iL_0\tau_2} F_{0,\alpha} \rangle_0, \quad (23)$$

We will only look at $I_2$ for now. Since the bare force-force correlation function is $\mathcal{O}(d^2)$, we need $I_{2n}$ to be $o(d^2)$. Each factor of $e^{iL_0\tau} F_{0,\alpha}$ imparts a time dependence only to coordinates $\mathbf{u}_{j>0}$ and the set $\mathbf{u}_{0,\alpha}^{\perp}$ (the coordinates of particle 0 orthogonal to the $\alpha$ direction) with no $p_{0,\alpha}$ dependence. Thus $O_F e^{iL_0\tau_2} F_{0,\alpha} = 0$ and $O_P e^{iL_0\tau_2} F_{0,\alpha} = -\frac{p_{0,\alpha}(0)}{m} \tilde{k}_\alpha(\tau_2)$. One can continue this procedure (ignoring the future action of $\nabla_{0,\alpha}$ on $\tilde{k}_\alpha$ and assuming $\langle F_{0,\alpha} \rangle_0 = 0$, in the spirit of keeping terms with derivatives of no higher order than that of $\tilde{k}_\alpha$), yielding

$$G_2 = -\frac{1}{m} \langle \tilde{F}_{0,\alpha}(0) \tilde{F}_{0,\alpha}(t-\tau_1) [\tilde{k}_\alpha(t) - \langle \tilde{k}_\alpha(t) \rangle_0] \rangle_0. \quad (24)$$

This term is $\mathcal{O}(d^{3/2})$. A proof that all $I_{2n}$ are subleading follows from considering the additional factors of $F_\alpha^\alpha$ that pair with factors of $\frac{1}{m}$ to bound the $d$-dependence, yielding a scaling $G_n \sim d^{(2-n/4)}$ for n even and 0 for n odd.

By translational invariance, and the fact that no $I_{2n}$ terms survive and thus no explicit $p_{0,\alpha}$ dependence survives, then Eq.4 of the main text holds exactly, with time evolution of the random force given by the unperturbed dynamics, as long as $d \to \infty$. It is amusing to compare this with the three dimensional case treated by Mazur and Oppenheim of a heavy particle immersed in a bath of light particles. In their case, the projected dynamics conspires to produce corrections to a frictional memory term (the clamped particle bare force-force correlator) that vanishes only at *long times* if the mass ratio of the tagged particle to that of the bath particles is large. In our case we also recover a simple generalized Langevin equation (GLE) of the same form (with a slightly different definition of the special coordinate) where the corrections vanish for *any* mass ratio for *all* times if $d \to \infty$.

Lastly, note that if we take as the tagged variable the full displacement $\mathbf{u}_0(t)$ instead of the displacement component $u_{0,\alpha}(t)$, then the expansion of the memory kernel would lead to terms that are not subleading with $d$. To see this, one can reconsider the calculation of $G_2(t,\tau_1,\tau_2)$ with the vector force on the tagged particle. The calculation is similar, but an extra unconstrained summation over particle direction renders the leading correction of order $d^{5/2}$ instead of $d^{3/2}$, and thus non-negligible in the $d \to \infty$ limit. This fact clearly illustrates the importance of choosing the correct variable in the derivation of the closed equations for the infinite dimensional fluid.

## V. NEWTONIAN TWO-PARTICLE PROCESS

We now generalize the one particle analysis for a pair of particles. For concreteness of notation, we label the two particles under consideration as 0 and 1. We follow

the analysis of Deutch and Oppenheim [4]. This analysis needs to be modified because in our case we must define the projection operator as

$$\mathcal{P}_2 A = \frac{1}{Z_2}\int\left(\prod_{i=2}^{N} d\mathbf{R}_i \prod_{i=2}^{N} d\mathbf{p}_i\right) d\mathbf{p}_{0,\alpha}^{\perp} d\mathbf{p}_{1,\alpha}^{\perp} \cdot d\mathbf{R}_{0,\alpha}^{\perp} d\mathbf{R}_{1,\alpha}^{\perp} A \exp(-\beta H_0) = \langle A\rangle_2, \qquad (25)$$

where $d\mathbf{p}_{i,\alpha}^{\perp} = \prod_{\nu\neq\alpha} dp_{i,\nu}$, $d\mathbf{R}_{i,\alpha}^{\perp} = \prod_{\nu\neq\alpha} dR_{i,\nu}$, $Z_2$ is defined, as usual, as the integrand above with $A = 1$, and $H_2 = \sum_{i>j} v(R_{ij}) + \sum_{j>1}\frac{\boldsymbol{p}_j^2}{2m} + \sum_{\nu\neq\alpha}\frac{p_{0,\nu}^2 + p_{1,\nu}^2}{2m}$. Note that this differs from the projector defined by Deutch and Oppenheim because all components of the coordinated of the two "tagged" particles 0 and 1 are averaged over aside from one arbitrary direction $\alpha$, whereas in the standard approach the averaging completely excludes the coordinates and momenta of the chosen pair of particles. This difference necessitates a small but crucial modification of the approach as outlined below, as well as a careful comparison of the final averaging with the standard configurational averaging, as discussed in the next section.

Consider the Newtonian equation of motion

$$\dot{p}_{0,\alpha} = F_{01,\alpha}(\mathbf{R}_{01}(t)) + \sum_{j>1} F_{0j,\alpha}(\mathbf{R}_{0j}(t))$$
$$\text{with } F_{0i,\alpha} = -\nabla_\alpha v(\boldsymbol{R}_{0i}(t)) \text{ for all } i \qquad (26)$$

Within the standard approach to the dynamics of a pair of tagged particles, there is no need to separate the force on a tagged particle into its contribution from the other tagged particle and the remaining particles. Here, this splitting is necessary as otherwise, given the form of our projection operator, the treatment of the direct dynamics becomes unduly complicated. We use the same identity as used in the previous section, namely $e^{(A+B)t} = e^{At} + \int_0^t e^{A(t-\tau)} B e^{(A+B)\tau} d\tau$ with $A = iL$, $B = \mathcal{P}_2 iL$, $L = \frac{p_{0,\alpha}}{m}\nabla_{0,\alpha} + \frac{p_{1,\alpha}}{m}\nabla_{1,\alpha} + F_{0,\alpha}\nabla_{p_{0,\alpha}} + F_{1,\alpha}\nabla_{p_{1,\alpha}} + iL_2$, and $iL_2$ defined from $H_2$ as given above, but we apply this identity *only* to the term $\sum_{j>1} F_{0j,\alpha}(\mathbf{R}_{0j}(t))$, while the term $F_{01,\alpha}(\mathbf{R}_{01}(t))$ evolves completely with the standard Newtonian dynamics generated by $\exp(iLt)$. Making use of the fact that $\mathcal{P}_2 iL_2 B = 0$ for any $B$, and defining the fluctuating force term for tagged particle $n$ $K_{n,\alpha}^{\dagger}(t) = \exp\left(i(1-\mathcal{P}_2)Lt\right)\sum_{j>1} F_{nj,\alpha}(\mathbf{R}_{0j}(0))$ along with the definition $\hat{\Delta}_n = \left[\nabla_{p_{n,\alpha}} - \frac{\beta}{m} p_{n,\alpha}\right]$, we find the coupled equations

$$\begin{aligned}\dot{p}_{0,\alpha}(t) =& F_{01,\alpha}(t) + K_{0,\alpha}^{\dagger}(t) \\ &+ \int_0^t d\tau e^{iL(t-\tau)} \hat{\Delta}_0 \langle F_{0,\alpha} K_{0,\alpha}^{\dagger}(\tau)\rangle_2 \\ &+ \int_0^t d\tau e^{iL(t-\tau)} \hat{\Delta}_1 \langle F_{1,\alpha} K_{0,\alpha}^{\dagger}(\tau)\rangle_2, \qquad (27)\\ \dot{p}_{1,\alpha}(t) =& F_{10,\alpha}(t) + K_{1,\alpha}^{\dagger}(t) \\ &+ \int_0^t d\tau e^{iL(t-\tau)} \hat{\Delta}_0 \langle F_{1,\alpha} K_{0,\alpha}^{\dagger}(\tau)\rangle_2 \\ &+ \int_0^t d\tau e^{iL(t-\tau)} \hat{\Delta}_1 \langle F_{1,\alpha} K_{1,\alpha}^{\dagger}(\tau)\rangle_2. \qquad (28)\end{aligned}$$

Note that $\langle K_{n,\alpha}^{\dagger}(0)\rangle_2 = 0$. In addition, note that the memory term is *unbalanced*; the correlations involve the *total* force on a tagged particle, e.g. $F_{0,\alpha} = F_{01,\alpha}(\boldsymbol{R}_{01}) + \sum_{j>1} F_{0j,\alpha}(\mathbf{R}_{0j})$ and the fluctuating force $K_{n,\alpha}^{\dagger}(t)$ which excludes the interactions between the two tagged particles (0 and 1). Lastly, note that these equations appear to be coupled through a friction (memory) matrix. The latter two aspects greatly simplify in $d = \infty$. Other simplifications occur in a manner outlined in the previous section on the one-particle process.

As discussed in the main text, in infinite dimensions all off-diagonal terms in the frictional memory functions may be dropped because they involve correlations between pairs of particles that are distinct and thus uncorrelated. This means that we may remove the off-diagonal terms in the memory matrix as subleading, and, in addition, ignore $\langle F_{1,\alpha} K_{0,\alpha}^{\dagger}(\tau)\rangle_2$ and $\langle F_{0,\alpha} K_{1,\alpha}^{\dagger}(\tau)\rangle_2$ since both contain only either terms of off-diagonal nature or terms of even weaker correlation. Finally, following the same procedure outlined for the one particle case, for $d \to \infty$ an expansion in orders of powers of $d$ shows that to leading order one can drop the projected dynamics in both the fluctuating force and memory tensor. The leading order terms that now appear in the fluctuating force and memory terms are functions of $\tilde{\boldsymbol{R}}_{ij}$, where motion along $\alpha$ is blocked for the tagged particles.

Thus we arrive at the equations

$$m\ddot{u}_{0,\alpha}(t) = -v'(R_{01}(t))\delta_{\alpha,\gamma} + \tilde{F}_{0,\alpha}(t) - \beta\int_0^t \langle \tilde{F}_{0,\alpha}(0)\tilde{F}_{0,\alpha}(\tau)\rangle_2 \dot{u}_0(t-\tau), \qquad (29a)$$

$$m\ddot{u}_{1,\alpha}(t) = v'(R_{01}(t))\delta_{\alpha,\gamma} + \tilde{F}_{1,\alpha}(t) - \beta\int_0^t \langle \tilde{F}_{1,\alpha}(0)\tilde{F}_{1,\alpha}(\tau)\rangle_2 \dot{u}_1(t-\tau), \qquad (29b)$$

where we have converted our notation for the fluctuating force from $K^{\dagger}$ to $\tilde{F}_{0,\alpha}$ as there is no potential confusion between the total force on a tagged particle and the fluctuating force. Note as well, that the equations above are valid for a general direction $\alpha$, however if $\alpha$ is chosen

along a direction other than the initial inter-particle one between the tagged pair, namely the direction labeled $\gamma$ defined as $\hat{\boldsymbol{e}}_\gamma \equiv \hat{\boldsymbol{R}}_{01}(0) = \frac{\mathbf{R}_0(0)-\mathbf{R}_1(0)}{|\mathbf{R}_0(0)-\mathbf{R}_1(0)|}$, then the leading direct force terms vanish in $d = \infty$. To arrive at the final closed theory, the same arguments concerning the restoration of the motion along the $\alpha$ direction put forward in the discussion of the 1-particle case may be made, which imply $\tilde{\boldsymbol{R}}_{ij}(t) \to \mathbf{R}_{ij}(t)$. Then, as justified in the next section, applying either $\langle\cdot\rangle_2$ or $\langle\cdot\rangle_0$ in Eq.29 makes a sub-leading difference, which allows replacement $\langle\cdot\rangle_2 \to \langle\cdot\rangle_0$ and finally making use of Eq. 7-9 of the main text, we arrive at Eq.10 in the main text.

## VI. NEGLIGIBLE DIFFERENCE BETWEEN $\mathcal{P}$ AND $\mathcal{P}_2$

The difference between the averages using $\mathcal{P} = \langle\cdot\rangle_0$ and $\mathcal{P}_2 = \langle\cdot\rangle_2$ comes from the different domains of integration over the configuration space of particle positions. Using the Boltzmann weight of Eq.13, the projection $\mathcal{P}$, after integrating out momentum, can be expressed as

$$\mathcal{P}\bullet = \frac{1}{\hat{Z}_0}\int_{\mathbb{S}_{d-1}} d\boldsymbol{R}_{01} e^{-\beta v(R_{01})} \cdot \prod_{(ij)\in E\backslash(01)} \int_{\mathbb{S}_{d-1}} d\boldsymbol{R}_{ij} e^{-\beta v(R_{ij})}\bullet, \tag{30}$$

where the integration over $d\boldsymbol{R}^{\perp}_{0,\alpha}$ is discarded by translation invariance and thus $\mathcal{P}$ is equivalent to the equilibrium thermal average. Similarly, the projection for the two particle computation is expressed as

$$\mathcal{P}_2\bullet = \frac{1}{Z_2^*}\int_{\mathbb{S}_{d-1}} d\boldsymbol{R}_{01}\delta(R_{01,\alpha} - R^*_\alpha) e^{-\beta v(R_{01})} \prod_{(ij)\in E\backslash(01)} \int_{\mathbb{S}_{d-1}} d\boldsymbol{R}_{ij} e^{-\beta v(R_{ij})}\bullet, \tag{31}$$

where $R^*_\alpha$ is the chosen fixed distance along direction $\alpha$ between the two particles and $Z_2^*$ depending on $R^*_\alpha$ is the adapted normalization factor.

By changing to polar coordinates, the restricted integration Eq.31 and its relation with $\mathcal{P}$ can be clearly illustrated because of the spherical symmetry of the integration domain $\mathbb{S}_{d-1}$ and the energy $v(R)$. We will use $\boldsymbol{R}$ for $\boldsymbol{R}_{01}(0)$ (the "(0)" is retained to emphasize the initial condition when considering dynamics) throughout this section for shortening the notation. The polar coordinates $(R, \phi_1, \phi_2, \ldots, \phi_{d-1})$ are defined in the following way, setting the direction $\alpha$ as the "first" direction by an arbitrary choice

$$\begin{aligned} R_\alpha \equiv R_1 &= R\cos\phi_1, \\ R_2 &= R\sin\phi_1\cos\phi_2, \\ R_3 &= R\sin\phi_1\sin\phi_2\cos\phi_3, \\ &\ldots \\ R_{d-1} &= R\sin\phi_1\sin\phi_2\ldots\sin\phi_{d-2}\cos\phi_{d-1}, \\ R_d &= R\sin\phi_1\sin\phi_2\ldots\sin\phi_{d-2}\sin\phi_{d-1}. \end{aligned} \tag{32}$$

The restricted integral

$$\int_{\mathbb{S}_{d-1}} d\boldsymbol{R}\delta(R_\alpha - R^*_\alpha) e^{-\beta v(R)}\bullet \tag{33}$$

is expressed in polar coordinates

$$\int_{|R-1|\lesssim d^{-1}} R^{d-1} dR \left(\prod_{s=1}^{d-2}\int_0^\pi d\phi_s (\sin\phi_s)^{d-1-s}\right) \int_0^{2\pi} d\phi_{d-1}\delta(R\cos\phi_1 - R^*_\alpha) e^{-\beta v(R)}\bullet. \tag{34}$$

Integrating first over $\phi_1$ leads to

$$\begin{aligned} &\int_{|R-1|\lesssim d^{-1}} R^{d-2} dR \left(\prod_{s=2}^{d-2}\int_0^\pi d\phi_s (\sin\phi_s)^{d-1-s}\right) \int_0^{2\pi} d\phi_{d-1} (\sin\phi_1^*)^{d-3} e^{-\beta v(R)}\bullet, \\ &\equiv \int_{\mathbb{S}_{d-2}} d\boldsymbol{R}^{\perp} (\sin\phi_1^*)^{d-3} e^{-\beta v(|\boldsymbol{R}^{\perp}|)}\bullet, \end{aligned} \tag{35}$$

where $\phi_1^*$ satisfies $\cos\phi_1^* = R^*_\alpha/R$. Note that $R^*_\alpha \sim d^{-1/2}$. To the leading order, we have $\phi_1^* \approx \pi/2 - R^*_\alpha/R$ and thus $\sin\phi_1^* \approx 1 - (R^*_\alpha/R)^2$, implying $(\sin\phi_1^*)^{d-3} \approx \exp(-d(R^*_\alpha/R)^2)$. Since $R = 1 + h/d$ with $h \sim 1$, we have to the leading order $(\sin\phi_1^*)^{d-3} \approx \exp(-dR^{*2}_\alpha)$ and the integration in Eq.33 becomes

$$e^{-dR^{*2}_\alpha}\int_{\mathbb{S}_{d-2}} d\boldsymbol{R}^{\perp} e^{-\beta v(|\boldsymbol{R}^{\perp}|)}\bullet. \tag{36}$$

This implies that $\mathcal{P}_2$ can be written as

$$\mathcal{P}_2\bullet = \frac{1}{\hat{Z}_2}\int_{\mathbb{S}_{d-2}} d\boldsymbol{R}^{\perp}_{01,\alpha} e^{-\beta v(R_{01})} \prod_{(ij)\in E\backslash(01)} \int_{\mathbb{S}_{d-1}} d\boldsymbol{R}_{ij} e^{-\beta v(R_{ij})}\bullet, \tag{37}$$

with the normalization factor $\hat{Z}_2 = e^{-dR^{*2}_\alpha}/Z_2^*$ no longer depending on $R^*_\alpha$. From Eq.36, we deduce that in the mean-field limit $d \to \infty$, the component of the particle distance along a fixed direction is actually given by a Gaussian distribution independent of the other directions. Thus, the projector $\mathcal{P}$ can be expressed, letting $A$ being an arbitrary physical quantity,

$$\mathcal{P}A = \int \sqrt{\frac{d}{\pi}} dR_\alpha e^{-dR^2_\alpha} (\mathcal{P}_2 A), \tag{38}$$

which explicitly shows that the difference between $\mathcal{P}A$ and $\mathcal{P}_2 A$ depends on how $A$ varies with $R_\alpha$ in the range from 0 to $\mathcal{O}(d^{-1/2})$. Any polynomial dependence, i.e. $|A(R_\alpha,\ldots) - A(R_\alpha = 0,\ldots)| \sim c|R_\alpha|^k$ gives rise to a difference

$$|\mathcal{P}A - \mathcal{P}_2 A| \sim \mathcal{O}(cd^{-k/2}). \quad (39)$$

In the case where $A$ is a force-force product, we can show that the modification made by varying $R_{01,\alpha}(0)(\equiv R_\alpha)$ from 0 to $\mathcal{O}(d^{-1/2})$ is quadratic in $R_\alpha$ and the the total modification in switching integration domains is of order $d^{-1/2}$. Let

$$A \hat{=} F_{0j,\alpha}(\tilde{\boldsymbol{R}}_{0j}(t))F_{0j,\alpha}(\tilde{\boldsymbol{R}}_{0j}(s)) \quad (40)$$

for $j \neq 1$, which simplifies for $d \to \infty$ (see the main text):

$$A \hat{=} \hat{R}_{0j,\alpha}(0)^2 v'(\tilde{R}_{0j}(t))v'(\tilde{R}_{0j}(s)). \quad (41)$$

To the leading order, we have

$$\tilde{R}_{0j} \equiv |\tilde{\boldsymbol{R}}_{0j}| \approx R_{0j}(0) + \hat{\boldsymbol{R}}_{0j}(0)\cdot(\tilde{\boldsymbol{u}}^{\perp}_{0,\alpha} - \tilde{\boldsymbol{u}}_j) + \boldsymbol{u}^2 \quad (42)$$

where the last symbolic term $\boldsymbol{u}^2$ concentrates on its typical value with negligible fluctuations and thus is effectively deterministic. Only $\tilde{y}_{0j} \hat{=} \hat{\boldsymbol{R}}_{0j}(0)\cdot(\tilde{\boldsymbol{u}}^{\perp}_{0,\alpha} - \tilde{\boldsymbol{u}}_j)$ depends non-trivially on the initial condition. Recall that the dynamics described by the Liouvillian $L_0$ implies that the evolution of $\tilde{y}_{0j}$ depends on $\boldsymbol{R}_{01}(0)(\equiv \boldsymbol{R})$ through

$$m\ddot{\tilde{y}}_{0j} = \ldots + \hat{\boldsymbol{R}}_{0j}(0)\cdot\hat{\boldsymbol{R}}^{\perp} v'(R + \tilde{y}_{01} + \boldsymbol{u}^2), \quad (43)$$

where the left-hand side can be replaced by $\zeta\dot{\tilde{y}}_{0j}$ when considering Brownian dynamics and we have used the self-averaging property of the $\tilde{y}$ variables. Using polar coordinates Eq.32 for $\boldsymbol{R}$, the last term in Eq.43 becomes

$$\sum_{\nu\geq 2}^{d} \hat{R}_{0j,\nu}(0)\sin\phi_1\left(\prod_{l=2}^{\nu-1}\sin\phi_l\right)(\cos\phi_\nu)^{\sum_{q=2}^{d-1}\delta_{q,\nu}} v'(R+...). \quad (44)$$

Here $\hat{R}_{0j,\nu}(0)$ is a scalar component of the initial relative vector between particles 0 and $j$. Then the modification on $\tilde{y}_{0j}$ due to the change of $R_\alpha$ from 0 to $R^*_\alpha \sim d^{-1/2}$ can be estimated by developing up to the leading order of $\sin\phi^*_1$ with $\phi^*_1$ satisfying $\cos\phi^*_1 = (R^*_\alpha/R)^2$. Recalling that $m \sim \zeta \sim d^2$, we arrive at

$$\begin{aligned}\delta\tilde{y}_{0j} &\sim \frac{1}{m}\left(\frac{R^*_\alpha}{R}\right)^2\left[\sum_{\nu\geq 2}^{d}\hat{R}_{0j,\nu}(0)\left(\prod_{l=2}^{\nu-1}\sin\phi_l\right)\right.\\ &\qquad\left.(\cos\phi_\nu)^{\sum_{q=2}^{d-1}\delta_{q,\nu}}\right]v'(R+...),\\ &= \frac{1}{m}\left(\frac{R^*_\alpha}{R}\right)^2\sum_{\nu\geq 2}^{d}\hat{R}_{0j,\nu}(0)\hat{x}_\nu v'(R+...)\\ &\text{with } \sum_{\nu\geq 2}^{d}\hat{x}_\nu \equiv 1, \end{aligned} \quad (45)$$

implying

$$\delta\tilde{y}_{0j} \sim d^{-2+\frac{1}{2}-\frac{1}{2}-\frac{1}{2}+1}R^{*2}_\alpha \sim d^{-3/2}R^{*2}_\alpha. \quad (46)$$

Then considering Eq.41, to the leading order, we have

$$|A(R^*_\alpha) - A(0)| \sim \hat{R}^2_{0j,\alpha} v'v''\delta\tilde{y}_{0j} \sim d^{1/2}R^{*2}_\alpha. \quad (47)$$

From Eq.39, the integrals over the force-force correlations differ by $\mathcal{O}(d^{-1/2})$, which is a sub-leading term compared to the correlation itself which is $\mathcal{O}(d)$. We conclude that the difference of the sum of diagonal terms of the force-force correlations, either computed using $\mathcal{P}$ or $\mathcal{P}_2$, is a sub-leading factor of $d$, negligible in the large $d$ limit.

We conclude this discussion by pointing out that the memory kernels in Eq.29 for the two particle process is identical to that in Eq.21 for the one particle process. The details for the passage from Eq.5 to Eq.7 in the main text are presented in Sec.IX.

## VII. BROWNIAN PROJECTION OPERATOR FORMALISM

The development of the projection operator formalism for a system evolving with Brownian dynamics is fundamentally similar to that of the formalism for a system evolving with Newtonian dynamics. However, there are some unique technical steps that we will point out.

We start from the equations of motion (Eq.1 of the main text) adapted to a system evolving with overdamped Brownian dynamics,

$$\zeta\dot{\boldsymbol{R}}_i = -\sum_{j(\neq i)}\boldsymbol{\nabla}_i v(\boldsymbol{R}_{ij}) + \boldsymbol{\xi}_i. \quad (48)$$

Like for Newtonian dynamics, the time evolution given by Eqs.48 can also be represented by a Liouville operator, $L$. In the present case, since the evolution equation involves a stochastic process, it is a stochastic Liouville operator [5]

$$L(t) = \frac{1}{\zeta}\sum_i(\mathbf{F}_i + \boldsymbol{\xi}_i(t) + T\boldsymbol{\nabla}_i)\cdot\boldsymbol{\nabla}_i, \quad (49)$$

where $\mathbf{F}_i = -\sum_{j(\neq i)}\boldsymbol{\nabla}_i v(\boldsymbol{R}_{ij})$ and the second derivative term originates from the Ito convention. The important technical feature of the stochastic Liouville operator is its explicit dependence on time, coming from the time dependence of a given noise realization. We note that in contrast to the more usual Liouville operator corresponding to the Newtonian equations of motion, Eq. (14), operator (49) is customarily defined without the imaginary factor $i$.

The time dependence of the stochastic Liouvillian implies that the corresponding evolution operator is given by a time-ordered exponential. As lucidly explained in Sec. 7.7 of Ref. [6], the Liouville operators in the evolution operator $U[L](t;t')$ should be ordered from left to

right as time increases, *i.e.*

$$U[L](t;t') = \exp\left(\int_{t'}^{t} dt_1 L(t_1)\right). \qquad (50)$$

Correspondingly,

$$\partial_t U[L](t;t') = U[L](t;t')L(t). \qquad (51)$$

As explained in the main text, the crucial step is to recognize that we should consider a component of the equation of motion for tagged particle, labeled 0, along an arbitrary direction $\alpha$,

$$\zeta \dot{R}_{0,\alpha} = F_{0,\alpha} + \xi_{0,\alpha}. \qquad (52)$$

We note that this equation is not closed in that the evolution of $R_{0,\alpha}$ depends on other coordinates of particle 0 and on the coordinates of all the other particles.

To analyze Eq.52, we start with a definition of the projection operator, $\mathcal{P}$, which is the close analog of the projection operator (16) introduced in Sec. IV,

$$\begin{aligned}\mathcal{P}X &\equiv \langle X\rangle_0 \\ &\equiv \left\langle \frac{\int d\mathbf{R}_0^{\perp} d\mathbf{R}_1 \ldots d\mathbf{R}_N e^{-\beta\sum_{i\neq j} v(R_{ij})} X}{\int d\mathbf{R}_0^{\perp} d\mathbf{R}_1 \ldots d\mathbf{R}_N e^{-\beta\sum_{i\neq j} v(R_{ij})}} \right\rangle_{\boldsymbol{\xi}_1,\ldots,\boldsymbol{\xi}_N}\end{aligned} \qquad (53)$$

where $d\mathbf{R}_0^{\perp}$ denotes the integration over all the components of the coordinate vector of the tagged particle except for the specific component of interest, $\langle\ldots\rangle_{\boldsymbol{\xi}_1,\ldots,\boldsymbol{\xi}_N}$ denotes averaging over the noise associated with the *all* the particles, including the tagged particle. Note that there is no averaging over the position of the tagged particle along the special selected direction. However, due to translational invariance if $X$ depends only on the relative positions of the particles along the selected direction, *i.e.* $R_{0,\alpha} - R_{i,\alpha}$, then $\mathcal{P}X$ is independent of the specific component of the coordinate vector of the tagged particle.

We use the projection operator (53) to project the force due to other degrees of freedom on the space spanned by the selected coordinate of the tagged particle. We also use it to define the irreducible Liouville operator $L^{\text{irr}}$, which is the analogue of the projected Liouvillian "$(1-\mathcal{P})iL$" introduced in Sec. IV,

$$L^{\text{irr}} = L - \frac{1}{\gamma}\left(F_{0,\alpha} + \xi_{0,\alpha} + T\nabla_{0,\alpha}\right)\mathcal{P}\nabla_{0,\alpha} = L - \delta L. \qquad (54)$$

Next, we generalize the identity (17) to time-dependent Liouville operators,

$$\begin{aligned}U[L^{\text{irr}}](t;0) &= U[L](t;0) \\ &\quad - \int_0^t d\tau U[L](\tau;0)\delta L(\tau) U[L^{\text{irr}}](t;\tau).\end{aligned} \qquad (55)$$

We use Eq. (55) to rewrite the $\alpha$ component of the force on the tagged particle as

$$\begin{aligned}F_{0,\alpha}(t) &\equiv U[L](t;0)F_{0,\alpha} = U[L^{\text{irr}}](t;0)F_{0,\alpha} \\ &\quad + \int_0^t d\tau\, U[L](\tau;0)\,\delta L(\tau)\, U[L^{\text{irr}}](t;\tau)F_{0,\alpha}.\end{aligned} \qquad (56)$$

The first part of the right-hand side of Eq.56 is the fluctuating force and the second part is the memory function term. To demonstrate the latter, we note that integration by parts leads to

$$\begin{aligned}&\delta L(\tau) U[L^{\text{irr}}](t;\tau)F_{0,\alpha} \\ &= -\frac{\beta}{\zeta}\left(F_{0,\alpha} + \xi_{0,\alpha}\right)\mathcal{P}F_{0,\alpha}U[L^{\text{irr}}](t;\tau)F_{0,\alpha} \\ &= -\dot{R}_{0,\alpha}\beta\mathcal{P}F_{0,\alpha}U[L^{\text{irr}}](t;\tau)F_{0,\alpha},\end{aligned} \qquad (57)$$

where we also used the fact that for a variable $X$ that depends only on relative coordinates along the selected direction then $\mathcal{P}X$ is independent of $R_{0,\alpha}$.

Thus, the second term in Eq. (56) gives

$$\begin{aligned}&-\int_0^t d\tau\, U[L](\tau;0)\dot{R}_{0,\alpha}\beta\mathcal{P}F_{0,\alpha}U[L^{\text{irr}}](t;\tau)F_{0,\alpha} \\ &= -\int_0^t d\tau\, \dot{R}_{0,\alpha}(\tau)\beta\mathcal{P}F_{0,\alpha}(\tau)U[L^{\text{irr}}](t;\tau)F_{0,\alpha}(\tau).\end{aligned} \qquad (58)$$

We note that in principle in the projection in the second line should be performed with the selected coordinate of the tagged particle fixed at its position at time $\tau$ and $R_{0,\alpha}$ everywhere to the right of $\mathcal{P}$ should also be taken at time $\tau$. However we also note that the whole expression to the right of $\dot{R}_{0,\alpha}(\tau)$ is translationally invariant in space and (after averaging over all components of the noise) in time. Thus,

$$\begin{aligned}&\beta\mathcal{P}F_{0,\alpha}(\tau)U[\mathcal{L}^{\text{irr}}](t;\tau)F_{0,\alpha}(\tau) \\ &= \beta\mathcal{P}F_{0,\alpha}U[\mathcal{L}^{\text{irr}}](t-\tau;0)F_{0,\alpha} \\ &\equiv \beta\left\langle F_{0,\alpha}^{\dagger}(0)F_{0,\alpha}^{\dagger}(t-\tau)\right\rangle_0 = M^{\text{irr}}(t-\tau),\end{aligned} \qquad (59)$$

where we introduced fluctuating force $F_{0,\alpha}^{\dagger}$ evolving with the irreducible dynamics,

$$F_{0,\alpha}^{\dagger}(t) = U[L^{\text{irr}}](t;0)F_{0,\alpha}. \qquad (60)$$

and so-called irreducible memory function $M^{\text{irr}}$ that describes the internal friction for a Brownian system.

Now we show that the fluctuating force and memory function simplify in the same way as in the Newtonian case. First, we consider the fluctuating force: at short times we have

$$\begin{aligned}F_{0,\alpha}^{\dagger}(t) &\approx F_{0,\alpha} + tL^{\text{irr}}F_{0,\alpha} \\ &= F_{0,\alpha} + t\left[\frac{1}{\zeta}\left(F_{0,\alpha} + \xi_{0,\alpha} + T\nabla_{0,\alpha}\right)\mathcal{Q}\nabla_{0,\alpha}\right. \\ &\quad + \frac{1}{\zeta}\left(\mathbf{F}_0^{\perp} + \boldsymbol{\xi}_0^{\perp}(t) + T\boldsymbol{\nabla}_{\mathbf{R}_0^{\perp}}\right)\cdot\boldsymbol{\nabla}_{\mathbf{R}_0^{\perp}} \\ &\quad \left. + \frac{1}{\zeta}\sum_{i\geq 1}\left(\mathbf{F}_i + \boldsymbol{\xi}_i(t) + T\boldsymbol{\nabla}_{\mathbf{R}_i}\right)\cdot\boldsymbol{\nabla}_{\mathbf{R}_i}\right]F_{0,\alpha},\end{aligned} \qquad (61)$$

where $\mathcal{Q} = \mathcal{I} - \mathcal{P}$ is the orthogonal projection operator and superscript $^{\perp}$ indicates components orthogonal to the selected component $\alpha$. One can show that the

the first term in square brackets on the right-hand-side is $\mathcal{O}(d^{1/2})$ whereas each of the remaining two terms is $\mathcal{O}(d^1)$. Thus, the first term is negligible and in the expression for the fluctuating force one can replace the irreducible operator $L^{\mathrm{irr}}$ by the operator

$$L^0 = \frac{1}{\zeta}\left(\mathbf{F}_0^{\perp} + \boldsymbol{\xi}_0^{\perp}(t) + T\boldsymbol{\nabla}_{\mathbf{R}_0^{\perp}}\right)\cdot\boldsymbol{\nabla}_{\mathbf{R}_0^{\perp}} + \frac{1}{\zeta}\sum_{i\geq 1}\left(\mathbf{F}_i + \boldsymbol{\xi}_i(t) + T\boldsymbol{\nabla}_{\mathbf{R}_i}\right)\cdot\boldsymbol{\nabla}_{\mathbf{R}_i}. \tag{62}$$

The operator (62) is the close analogue of the unperturbed Liouvillian "$iL_0$" introduced in Sec. IV, see Eq. (15). This operator describes the evolution of all the degrees of freedom except for the selected coordinate of the tagged particle, which remains blocked. This shows that, like in the Newtonian case, the fluctuating force $F_{0,\alpha}^{\dagger}(t)$, Eq.60, evolves due to motion of all the other degrees of freedom while the selected coordinate is kept unchanged,

$$F_{0,\alpha}^{\dagger}(t) = \tilde{F}_{0,\alpha}(t) \equiv U[L^0](t;0)F_{0,\alpha}. \tag{63}$$

where notation $\tilde{F}_{0,\alpha}$ is borrowed from Sec. IV to denotes the force that evolves according to Brownian dynamics with the $\alpha$ coordinate of the tagged particle blocked.

Likewise, the expansion of the memory function works similarly to that in the Newtonian case, see Eqs. 21-23. We have

$$M^{\mathrm{irr}}(t) = \beta\left\langle F_{0,\alpha}U[L^{\mathrm{irr}}](t;0)F_{0,\alpha}\right\rangle_0 = \left\langle F_{0,\alpha}U[L^0](t;0)F_{0,\alpha}\right\rangle_0 + \int_0^t d\tau G_2^{\mathrm{irr}}(t;\tau) + ... \tag{64}$$

where

$$G_2^{\mathrm{irr}}(t;\tau) = \left\langle F_{0,\alpha}U[L^0](\tau;0)\delta L^0(\tau)U[L^0](t;\tau)F_{0,\alpha}\right\rangle_0 \tag{65}$$

and $\delta L^0 = L^{\mathrm{irr}} - L^0$. $G_2^{\mathrm{irr}}$ can be analyzed similarly to the above outlined analysis of the fluctuating force. The result is that $G_2^{\mathrm{irr}}$ and other terms in (64) involving $\delta L^0$ can be neglected.

The end result is that the evolution of the $\alpha$ component of the tagged particle position vector is given by the following equation

$$\zeta\dot{R}_{0,\alpha}(t) = \tilde{F}_{0,\alpha}(t) - \beta\int_0^t d\tau\left\langle\tilde{F}_{0,\alpha}(\tau)\tilde{F}_{0,\alpha}(t)\right\rangle_0\dot{R}_{0,\alpha}(\tau) + \xi_{0,\alpha}(t). \tag{66}$$

We note that in contrast to Eq. 52, the above equation is closed in that the evolution of component $\alpha$ of the coordinate vector of particle 0 is due to a well defined stochastic force $\tilde{F}_{0,\alpha}$. In the rest of this section we argue that in the large dimensional limit this stochastic force can be further simplified.

The specific arguments are similar to those described in detail in other sections (detailed in Sec.X). First, we note that the dominant term in the memory function originates from the so-called diagonal terms,

$$M^{\mathrm{irr}}(t) = \beta\left\langle\tilde{F}_{0,\alpha}(0)\tilde{F}_{0,\alpha}(t)\right\rangle_0 = \sum_i\beta\left\langle\tilde{F}_{0i,\alpha}(0)\tilde{F}_{0i,\alpha}(t)\right\rangle_0, \tag{67}$$

where $F_{0i,\alpha}(t)$ is the $\alpha$ component of the force acting on the tagged particle due to particle $i$, evolving due to the motion of all other particles while the $\alpha$ coordinate of the tagged particle is blocked. Second, we note that in the expression at the right-hand-side of Eq.67 we can replace the dynamics with the $\alpha$ coordinate being blocked by the full dynamics of the system,

$$M^{\mathrm{irr}}(t) = \sum_i\beta\left\langle\tilde{F}_{0i,\alpha}(0)\tilde{F}_{0i,\alpha}(t)\right\rangle_0 = \sum_i\beta\left\langle F_{0i,\alpha}(0)F_{0i,\alpha}(t)\right\rangle. \tag{68}$$

Third, we note that in the final expression (68), $\alpha$ is an arbitrary direction and due to rotational invariance we can average over all possible $\alpha$'s, which results in the following expression for the memory function,

$$M^{\mathrm{irr}}(t) = \sum_i\beta\left\langle F_{0i,\alpha}(0)F_{0i,\alpha}(t)\right\rangle = d^{-1}\sum_i\beta\left\langle\mathbf{F}_{0i,\alpha}(0)\cdot\mathbf{F}_{0i,\alpha}(t)\right\rangle. \tag{69}$$

We close this section observing that the final expression (69) for the irreducible memory function implies that in order to calculate the memory function we need to analyze the relative dynamics of a pair of particles, *e.g.* the dynamics of particles 0 and 1. This will be done in the next section.

## VIII. BROWNIAN TWO-PARTICLE PROCESS

First, we note that to evaluate the memory function (69) we need to analyze trajectories of particles 0 and 1 that start at the initial time, $t = 0$, within each other's interaction range (to make the force at the initial time non-vanishing) and end at time $t$ also within each other's interaction range. In the large dimensional limit the displacements of these two particles between the initial time and the final time are on a scale $d^{-1}$, *i.e.* for $i = 0, 1$, $\boldsymbol{u}_i^2 \sim d^{-1}$ with $\boldsymbol{u}_i \hat{=} \boldsymbol{R}_i(t) - \boldsymbol{R}_i(0)$, and accordingly on a scale $1/d$ for a given component, i.e. $u_{i,\mu} \sim d^{-1}$.

From the physical point of view there is a difference between the single-particle motion considered in the previous section and the two-particle motion considered in the present section. In principle, in both cases the motion of a given particle is unbounded (as it should be in a fluid). However, in the present section we are only interested in these parts of the two-particle trajectories that contribute to the memory function. During these parts

of the two-particle trajectories the displacements of the two particles are on a scale $d^{-1}$.

Initially, our variables of interest will be components of the coordinate vectors of particles 0 and 1 along an arbitrary direction $\alpha$. Subsequently, we will specify this direction to be along the direction along the initial inter-particle vector $\mathbf{R}_{01}(0) = \mathbf{R}_0(0) - \mathbf{R}_1(0)$, referred to in the main text as the $\gamma$ direction, $\hat{\boldsymbol{e}}_\gamma = \hat{\boldsymbol{R}}_{01}(0)$.

We start by writing down equations of motion for $\alpha$ components of the coordinate vectors of particles 0 and 1,

$$\zeta \dot{R}_{0,\alpha} = F_{01,\alpha} + \sum_{j\geq 2} F_{0j,\alpha} + \xi_{0,\alpha}, \tag{70}$$

$$\zeta \dot{R}_{1,\alpha} = F_{10,\alpha} + \sum_{j\geq 2} F_{1j,\alpha} + \xi_{1,\alpha}. \tag{71}$$

We note that in Eqs.70-71 we decomposed the forces acting on particles 0 and 1 to separate the direct force between these particles from forces due to all other particles of the fluid. We note that, as argued in Sec. II, in the $d \to \infty$ limit the particles interacting with particle 0 are different from the particles interacting with particle 1.

In the following we will present the analysis of Eq.70. Eq.71 can be analyzed in the same way.

We define the two-particle projection operator, $\mathcal{P}_2$, as follows

$$\mathcal{P}_2 X \equiv \left< X \right>_2 \equiv \left< \frac{\int d\mathbf{R}_0^\perp d\mathbf{R}_1^\perp d\mathbf{R}_2 \dots d\mathbf{R}_N e^{-\beta \sum_{i\neq j} v(R_{ij})} X}{\int d\mathbf{R}_0^\perp d\mathbf{R}_1^\perp d\mathbf{R}_2 \dots d\mathbf{R}_N e^{-\beta \sum_{i\neq j} v(R_{ij})}} \right>_{\boldsymbol{\xi}_1,\dots,\boldsymbol{\xi}_N} \tag{72}$$

where $d\mathbf{R}_i^\perp$, $i = 0, 1$ denotes the integration over all the components of the coordinate vector of particle $i$ perpendicular to the direction of interest $\alpha$. The projection operator (72) is the close analogue of projection operator (25) introduced in the section on Newtonian two-particle dynamics.

We use the projection operator (72) to define the two particle irreducible Liouville operator $L^{2\mathrm{irr}}$, which for Brownian dynamics plays the role of the two-particle projected Liouvillian,

$$L^{2\mathrm{irr}} = L - \frac{1}{\gamma}\left(F_{0,\alpha} + \xi_{0,\alpha} + T\nabla_{0,\alpha}\right)\mathcal{P}_2\nabla_{0,\alpha} - \frac{1}{\gamma}\left(F_{1,\alpha} + \xi_{1,\alpha} + T\nabla_{1,\alpha}\right)\mathcal{P}_2\nabla_{1,\alpha} = L - \delta L^2. \tag{73}$$

We use the two particle irreducible Liouville operator (73) to rewrite the $\alpha$ component of the force on particle 0 due to *other* particles as

$$\sum_{j\geq 2} F_{0j,\alpha}(t) \equiv U[L](t;0)\sum_{j\geq 2} F_{0j,\alpha} = U[L^{2\mathrm{irr}}](t;0)\sum_{j\geq 2} F_{0j,\alpha} + \int_0^t d\tau\, U[L](\tau;0)\,\delta L^2(\tau)\,U[L^{2\mathrm{irr}}](t;\tau)\sum_{j\geq 2} F_{0j,\alpha}. \tag{74}$$

Again, the first part of the right-hand-side of Eq. (74) is the fluctuating force and the second part is the memory function term. To show the latter, we note that

$$\delta L^2(\tau) U[L^{2\mathrm{irr}}](t;\tau)\sum_{j\geq 2} F_{0j,\alpha} = \frac{1}{\zeta}\left(F_{0,\alpha} + \xi_{0,\alpha} + T\nabla_{0,\alpha}\right)\mathcal{P}_2\nabla_{0,\alpha} U[L^{2\mathrm{irr}}](t;\tau)\sum_{j\geq 2} F_{0j,\alpha} + \frac{1}{\zeta}\left(F_{1,\alpha} + \xi_{1,\alpha} + T\nabla_{1,\alpha}\right)\mathcal{P}_2\nabla_{1,\alpha} U[L^{2\mathrm{irr}}](t;\tau)\sum_{j\geq 2} F_{0j,\alpha}. \tag{75}$$

Then, integration by parts leads to

$$\delta L^2(\tau) U[L^{2\mathrm{irr}}](t;\tau)\sum_{j\geq 2} F_{0j,\alpha} = -\frac{\beta}{\zeta}\left(F_{0,\alpha} + \xi_{0,\alpha} + T\nabla_{0,\alpha}\right)\mathcal{P}_2 F_{0,\alpha} U[L^{2\mathrm{irr}}](t;\tau)\sum_{j\geq 2} F_{0j,\alpha} - \frac{\beta}{\zeta}\left(F_{1,\alpha} + \xi_{1,\alpha} + T\nabla_{1,\alpha}\right)\mathcal{P}_2 F_{1,\alpha} U[L^{2\mathrm{irr}}](t;\tau)\sum_{j\geq 2} F_{0j,\alpha}. \tag{76}$$

Eq. (76) is considerably more complicated than the corresponding equation at the one-particle level, Eq. (57). The differences between these two equations parallel those between two-particle and one-particle memory function terms in the case of Newtonian dynamics. First, in principle we need to keep gradient terms $T\nabla_{i,\alpha}$, $i = 0, 1$, which implies that the memory function term cannot be fully interpreted as the time delayed friction. Second, expressions $\mathcal{P}_2 F_{i,\alpha} U[L^{2\mathrm{irr}}](t;\tau)\sum_{j\geq 2} F_{0j,\alpha}$, $i = 0, 1$, are unbalanced in that they involve correlations between forces due to *other* particles at time $t$ and forces due to *all* the particles at an earlier time. Third, we have a cross term which correlates forces acting on particle 0 at time $t$ and on particle 1 at an earlier time.

As for Newtonian dynamics, in the limit $d \to \infty$ all these complications disappear. In fact, the arguments used in the Newtonian dynamics derivation can be used also here. At the end we find that expression (76) reproduces the one-particle memory function term,

$$U[L](\tau;0)\delta L^2(\tau) U[L^{2\mathrm{irr}}](t;\tau)\sum_{j\geq 2} F_{0j,\alpha} = -\dot{R}_{0,\alpha}(\tau)\mathcal{P}\sum_{j\geq 2} F_{0j,\alpha}(\tau) U[L^0](t;\tau)\sum_{j\geq 2} F_{0j,\alpha}(\tau). \tag{77}$$

Thus we find the following equation of motion for particle 0,

$$\zeta \dot{R}_{0,\alpha} = F_{01,\alpha}(R_{01}(t)) + \tilde{F}_{0,\alpha}(t) - \beta\int_0^t d\tau \left< \tilde{F}_{0,\alpha}(\tau)\tilde{F}_{0,\alpha}(t)\right>_0 \dot{R}_{0,\alpha}(\tau) + \xi_{0,\alpha}(t), \tag{78}$$

where $\tilde{F}_{0,\alpha}(t)$ and $\beta\left< \tilde{F}_{0,\alpha}(\tau)\tilde{F}_{0,\alpha}(t)\right>_0$ are the same quantities that we introduced in the previous section.

At this point we recall that during the two particle trajectories we are interested in particles 0 and 1 which

move very little, and $u_{i,\alpha}(t) = R_{i,\alpha}(t) - r_{i,\alpha}(0) \sim d^{-1}$. Furthermore, we recognize the fact that the direct force $F_{01,\alpha}(R_{01}(t))$ is only important along the direction of the original interparticle vector $\mathbf{R}_0(0) - \mathbf{R}_1(0)$ (the $\gamma$ direction). Finally, we recall that, as discussed in the main text and in the section on Newtonian two-particle process, the interparticle force along $\mathbf{R}_0(0) - \mathbf{R}_1(0)$ can be expressed in terms of relative displacements of particles 0 and 1 along the original interparticle vector and along all the other directions,

$$\begin{aligned}&\hat{\mathbf{R}}_{01}(0) \cdot \mathbf{F}_{01}(\boldsymbol{R}_{01}(t)) \\ &= -v'(R_{01}(0) + w_{01}(t) + \Delta_w(t)/2R_{01}(0)),\end{aligned} \quad (79)$$

where $w_{01}(t)$ and $\Delta_w(t)$ have the same meaning as in the main text and can be further analyzed in the same way.

The final result is the following equation of motion for fluctuating quantity $w_{01}(t)$,

$$\begin{aligned}&\zeta \dot{w}_{01} = -2v'(R_{01}(0) + w_{01}(t) + \Delta_u(t)/2R_{01}(0)) \\ &+\tilde{F}_{0,\gamma}(t) - \tilde{F}_{1,\gamma}(t) \quad (80) \\ &-\beta \int_0^t d\tau \left\langle \tilde{F}_{0,\gamma}(\tau)\tilde{F}_{0,\gamma}(t) \right\rangle_0 \dot{w}_{01}(\tau) + \xi_{0,\alpha}(t) - \xi_{1,\alpha}(t).\end{aligned}$$

This is the Brownian analogue of the two particle Newtonian equation, Eq. (11), in the main text.

## IX. CAVITY – ONE PARTICLE PROCESS

We consider the over-damped limit of Eq.1 of the main text and chose $u_{0,\alpha}$ as the cavity variable. We intend to derive the effective equilibrium dynamics of the cavity variable. Developing the interactions up to the first order in $u_{0,\alpha}$ in Eq.1 of the main text, we find for the cavity

$$\begin{aligned}\zeta \dot{u}_{0,\alpha} &= \xi_{0,\alpha}(t) - \sum_{j>0} \nabla_\alpha v(\boldsymbol{X}_{0j}^\alpha) - \sum_{j>0} \nabla_\alpha \nabla_\alpha v(\boldsymbol{X}_{0j}^\alpha) u_{0,\alpha} \\ &+\mathcal{O}(u_{0,\alpha}^2),\end{aligned} \quad (81)$$

and for the other degrees of freedom

$$\begin{aligned}\zeta \dot{u}_{0,\nu} &= \xi_{0,\nu}(t) - \sum_{j>0} \nabla_\nu v(\boldsymbol{X}_{0j}^\alpha) \\ &\quad - \sum_{j>0} \nabla_\alpha \nabla_\nu v(\boldsymbol{X}_{0j}^\alpha) u_{0,\alpha} + \mathcal{O}(u_{0,\alpha}^2), \\ \zeta \dot{u}_{j,\mu} &= \xi_{j,\mu}(t) - \sum_{i>0, i\neq j} \nabla_\mu v(\boldsymbol{R}_{ji}) - \nabla_\mu v(\boldsymbol{X}_{j0}^\alpha) \\ &\quad +\nabla_\alpha \nabla_\mu v(\boldsymbol{X}_{0j}^\alpha) u_{0,\alpha} + \mathcal{O}(u_{0,\alpha}^2),\end{aligned} \quad (82)$$

where $\nu \neq \alpha$ and $\boldsymbol{X}_{0j}^\alpha \hat{=} \boldsymbol{R}_{0j}(0) + \boldsymbol{u}_{0,\alpha}^\perp - \boldsymbol{u}_j$.

In general, we have $(\prod_{i=1}^n \nabla_{\mu_i})v \sim (\prod_{i=1}^n \hat{R}_{\mu_i})v^{(n)} \sim d^{n/2}$. Thus $\nabla_\alpha^n \nabla_\mu v(\boldsymbol{R}) u_{0,\alpha}^n \sim d^{-(n+1)/2} d^{n+1} d^{-n} \sim d^{(1-n)/2}$. We first discuss high orders of the cavity variable, $u_{0,\alpha}^n$, with $n > 1$. In this case, individual terms are of negative order of magnitude in $d$. In particular, we have $\log\left(\nabla_\alpha^n \nabla_\mu v(\boldsymbol{X}_{0j}^\alpha) u_{0,\alpha}^n\right) \leq -\frac{1}{2}\log d$, which implies the summation $\sum_j^{\sim d}$ is of order of magnitude in $d$ no larger than $d \times d^{(1-n)/2} \sim d^{(3-n)/2}$. Thus it is clear that high order ($n > 1$) terms in $u_{0,\alpha}$ scale at most as $d^{1/2}$, and hence are negligible in all terms in Eq.81 and Eq.82. The situation is slightly more complicated when $n = 1$. Note that we used $\sum_j^{\sim d} \sim d$ to estimate the upper bound when summing up terms, which is correct if individual terms are of the same sign. In the case when individual terms alternate in sign with equal probability, we should use $\sum_j^{\sim d} \sim d^{1/2}$ by the central limit theorem. When $n = 1$, individual terms such as $\nabla_\alpha \nabla_\mu v(\boldsymbol{R}) u_{0,\alpha} \sim 1$ are negligible. However when summing up over $j$, the order of magnitude depends on whether $\mu = \alpha$. In the case where $\mu = \nu \neq \alpha$, we have $\nabla_\alpha \nabla_\nu v \sim \hat{R}_{0j,\alpha} \hat{R}_{0j,\nu} v''$ which alternates in sign over all $j$ due to the fact that $\nu$ is orthogonal to $\alpha$. Thus the sum is of order $d^{1/2}$ which is subleading. When $\mu = \alpha$, i.e. the correction in Eq.81, we have $\nabla_\alpha^2 v \sim (\hat{R}_{0j,\alpha})^2 v''$ which is always positive thus the sum gives a linear correction of order $d$, the same order as the other terms in Eq.81. [7]

To summarize the above discussion, the interaction force acting on the cavity $u_{0,\alpha}$ can be accounted for exactly by retaining terms up to the first order in $u_{0,\alpha}$ and the trajectories of the non-cavity variables, namely $\boldsymbol{u}_{0,\alpha}^\perp$ and $\boldsymbol{u}_{j>0}$, receive negligible contributions from the motion of the cavity $u_{0,\alpha}$ when $d \to \infty$. Thus the dynamics of the non-cavity variables, when discarding the cavity-related perturbations, is associated with the real system potential energy $V = \sum_{i<j} v(\boldsymbol{R}_{ij})$, but subjected to the constraint that the tagged particle 0 is blocked in direction $\alpha$. The perturbation can be regarded as coming from a linear coupling with an "external field" $u_{0,\alpha}$ by $\Delta V = -\sum_{j>0} \nabla_\alpha v(\boldsymbol{X}_{0j}^\alpha) u_{0,\alpha}$. This perturbation gives rise to corrections $\delta \boldsymbol{u}_{0,\alpha}^\perp[u_{0,\alpha}]$ and $\delta \boldsymbol{u}_j[u_{0,\alpha}]$ which are negligible with respect to the non-perturbed trajectories denoted with an "tilde" by $\tilde{\boldsymbol{u}}_{0,\alpha}^\perp(t)$ and $\tilde{\boldsymbol{u}}_j(t)$. Nonetheless, the summed effect on the dynamics of $u_{0,\alpha}$ in Eq.81, which can be accounted for in linear response, is non-negligible.

Since we are interested in the equilibrium dynamics, we shall consider the equilibrium distribution of the initial configurations. We denote the entire equilibrium average as

$$\begin{aligned}\langle \cdot \rangle &= \frac{1}{Z} \int \prod_{i=0}^N \mathcal{D}[\boldsymbol{\xi}_i] d\boldsymbol{R}_i(0) \exp(-\beta V), \\ &\text{where } V = \sum_{0 \leq i<j \leq N} v(R_{ij}(0)).\end{aligned} \quad (83)$$

We introduce the equilibrium average of the non perturbed system

$$\langle \cdot \rangle_0 = \frac{1}{\hat{Z}_0} \int \mathcal{D}[\boldsymbol{\xi}_{0,\alpha}^\perp] \prod_{i=1}^N \mathcal{D}[\boldsymbol{\xi}_i] d\boldsymbol{R}_{0i}(0) \exp(-\beta V). \quad (84)$$

It is worth noticing that the equilibrium average over the real system initial condition coincides with the that

of the non-perturbed system, defined via Eq.82, when averaging over quantities that are translation-invariant (This has also been mentioned in Sec.VI, i.e. the equivalence between the equilibrium thermal average and $\mathcal{P}$). We use the same notation as in the main article, namely $\tilde{F}_{0,\mu} = -\sum_{j>0} \nabla_\mu v(\tilde{\boldsymbol{R}}_{0j}), \quad \mu = 1, 2 \ldots, d$ for the forces evaluated along the trajectories of the non-perturbed system and we denote $\tilde{k}_\alpha = \sum_{j>0} \nabla_\alpha^2 v(\tilde{\boldsymbol{R}}_{0j})$ with $\tilde{\boldsymbol{R}}_{0j} = \boldsymbol{R}_{0j}(0) + \tilde{\boldsymbol{u}}_{0,\alpha}^{\perp} - \tilde{\boldsymbol{u}}_j$.

Applying linear response to take into account the summed feedback effect on the dynamics of $u_{0,\alpha}$, we rewrite Eq.81, for one realization of the randomness, as

$$\zeta \dot{u}_{0,\alpha} = \xi_{0,\alpha}(t) + \tilde{F}_{0,\alpha} + \delta\tilde{F}_{0,\alpha} - (\tilde{k}_\alpha + \delta\tilde{k}_\alpha) u_{0,\alpha}, \tag{85}$$

where

$$\begin{aligned} \delta\tilde{F}_{0,\alpha}(t) &= \int_0^t ds \chi_F[\tilde{\boldsymbol{R}}](t,s) u_{0,\alpha}(s) \hat{=} \int_0^t ds \frac{\delta\tilde{F}_{0,\alpha}(t)}{\delta u_{0,\alpha}(s)}\bigg|_{\tilde{\boldsymbol{R}}} u_{0,\alpha}(s), \\ \delta\tilde{k}_\alpha(t) &= \int_0^t ds \frac{\delta\tilde{k}_\alpha(t)}{\delta u_{0,\alpha}(s)}\bigg|_{\tilde{\boldsymbol{R}}} u_{0,\alpha}(s). \end{aligned} \tag{86}$$

The correction $\delta\tilde{k}_\alpha \sim \mathcal{O}(u_{0,\alpha})$ can be dropped, as we only need to keep up to the first order in $u_{0,\alpha}$ in Eq.85. Eq.85 illustrates more transparently how the trajectory of the cavity variable is determined given one realization of the non-cavity trajectories. Now all non-cavity variable involved terms can be regarded as stochastic input, just as for the thermal noise $\xi_{0,\alpha}$, which defines the effective stochastic dynamics of $u_{0,\alpha}$. We can separate the non-cavity variables involved terms into their averages and the fluctuations, which leads to

$$\begin{aligned} \zeta \dot{u}_{0,\alpha} = \xi_{0,\alpha}(t) + \Big[\tilde{F}_{0,\alpha} - \langle \tilde{F}_{0,\alpha}\rangle_0\Big] + \int_0^t ds \langle \chi_F(t,s)\rangle_0 u_{0,\alpha}(s) - \langle \tilde{k}_\alpha\rangle_0 u_{0,\alpha} + \langle \tilde{F}_{0,\alpha}\rangle_0 \quad &\sim \mathcal{O}(d) \\ -(\tilde{k}_\alpha - \langle \tilde{k}_\alpha\rangle_0) u_{0,\alpha} + \int_0^t ds \big[\chi_F(t,s) - \langle \chi_F(t,s)\rangle_0\big] u_{0,\alpha}(s) \quad &\sim \mathcal{O}(d^{1/2}), \end{aligned} \tag{87}$$

where the second line represents the fluctuation of a sum over $\sim d$ weakly correlated terms, each of which has fluctuations of order one (as the average of the sum is order $d$ in the first line). Hence the second line is order $d^{1/2}$, which is sub-leading and thus can be dropped. Note that by symmetry of inverting the $\alpha$ direction, $\langle \tilde{F}_{0,\alpha}\rangle_0 = 0$ as well as individual terms that sum up to $\tilde{F}_{0,\alpha}$ and, as we showed above, the fluctuation $\tilde{F}_{0,\alpha} - \langle \tilde{F}_{0,\alpha}\rangle_0$ is order $d$ and non-negligible.

Applying the fluctuation-dissipation theorem for the averaged linear response $\langle \chi_F\rangle_0$ and integrating by parts leads to

$$\begin{aligned} &\zeta \dot{u}_{0,\alpha} = \xi_{0,\alpha} + \mathcal{F}_{0,\alpha}(t) - \beta \int_0^t ds \langle \mathcal{F}_{0,\alpha}(t)\mathcal{F}_{0,\alpha}(s)\rangle_0 \dot{u}_{0,\alpha}(s) + F_\alpha^{\text{eff}}(u_{0,\alpha}), \\ &\text{with} \quad \mathcal{F}_{0,\alpha} \hat{=} \tilde{F}_{0,\alpha} - \langle \tilde{F}_{0,\alpha}\rangle_0 \quad \text{and} \quad F_\alpha^{\text{eff}}(u_{0,\alpha}) = \langle \tilde{F}_{0,\alpha}(t)\rangle_0 - \langle \tilde{k}_\alpha(t)\rangle_0 u_{0,\alpha} + \beta \langle \big[\tilde{F}_{0,\alpha}(t) - \langle \tilde{F}_{0,\alpha}(t)\rangle_0\big]^2\rangle_0 u_{0,\alpha}(t). \end{aligned} \tag{88}$$

Now we are going to show $F_\alpha^{\text{eff}} = 0$. We have the partition function of the non perturbed system

$$\begin{aligned} \hat{Z}_0 &= \int \prod_{i>0} d\boldsymbol{R}_{0i} \exp\left(-\beta V\right), \\ V &= \sum_{i>0} v(\boldsymbol{R}_{0i}) + \sum_{0<i<j} v(\boldsymbol{R}_{0i} - \boldsymbol{R}_{0j}), \end{aligned} \tag{89}$$

which does not depend explicitly on $\boldsymbol{R}_0$. Thus the potential mean force $-\partial_{R_{0,\alpha}}\big[-\beta^{-1}\ln Z_0\big] = 0$ for all $\boldsymbol{R}_0$. By changing variables $\boldsymbol{R}_0 \to \boldsymbol{R}_0 + u_{0,\alpha}\hat{\boldsymbol{e}}_\alpha$, it is easy to verify that

$$\begin{aligned} &-\partial_{R_{0,\alpha}}\big[-\beta^{-1}\ln \hat{Z}_0\big]\Big|_{\boldsymbol{R}_0 + u_{0,\alpha}\hat{\boldsymbol{e}}_\alpha} \\ &\quad = F_\alpha^{\text{eff}}(u_{0,\alpha}) + \mathcal{O}(u_{0,\alpha}^2). \end{aligned} \tag{90}$$

As a result, $F_\alpha^{\text{eff}} = 0$.

We explicitly justify in the next section of the key step

for obtaining the final equation, which is

$$\langle \mathcal{F}_{0,\alpha}(t)\mathcal{F}_{0,\alpha}(s)\rangle_0 = \langle \tilde{F}_{0,\alpha}(t)\tilde{F}_{0,\alpha}(s)\rangle_0 \stackrel{d\to\infty}{=} \sum_{i>0}\langle \nabla_\alpha v(R_{0i}(t))\nabla_\alpha v(R_{0i}(s))\rangle \tag{91}$$

Namely we can neglect the off-diagonal terms and restore the true trajectories within the diagonal terms in the force-force correlation.

Now we can write the final version of the one particle effective process by promoting Eq.88 to a vector form, as the choice of $\alpha$ is completely arbitrary.

$$\zeta \dot{\boldsymbol{u}}_0 = \boldsymbol{\xi}_0 + \boldsymbol{\mathcal{F}}_0 - \beta\int_0^t ds \mathcal{M}(t-s)\dot{\boldsymbol{u}}_0(s), \quad \text{with} \quad \langle \mathcal{F}_{0,\mu}(t)\mathcal{F}_{0,\nu}(s)\rangle_{\mathcal{F}} = \delta_{\mu\nu}\mathcal{M}(t-s), \tag{92}$$

and the memory function carries the following physical meaning

$$\mathcal{M}(t-s) \stackrel{d\to\infty}{=} \frac{1}{d}\sum_{i>0}^{\sim d}\langle v'(R_{0i}(t))v'(R_{0i}(s))\rangle. \tag{93}$$

As we have discussed in the main text, the vector form above holds in any direction that is not correlated with the initial interparticle distances.

## X. DIAGONAL APPROXIMATION

The passage Eq.91 is the key step in all of our three derivations, which appears in the main text as the passage from Eq.5 to Eq.7. We explicitly justify this step adopting the overdumped dynamics without losing generality for the Newtonian dynamics case.

The force-force correlation $\langle \tilde{F}_{0,\alpha}(t)\tilde{F}_{0,\alpha}(s)\rangle_0$ is explicitly written

$$\begin{aligned}
&\langle \mathcal{F}_{0,\alpha}(t)\mathcal{F}_{0,\alpha}(s)\rangle_0 = \langle \tilde{F}_{0,\alpha}(t)\tilde{F}_{0,\alpha}(s)\rangle_0 \\
&\stackrel{d\to\infty}{=} \sum_{i,j}\langle \hat{R}_{0i,\alpha}(0)v'(\tilde{R}_{0i}(t))\hat{R}_{0j,\alpha}(0)v'(\tilde{R}_{0j}(s))\rangle_0 \\
&= \sum_{i,j}\langle \hat{R}_{0i,\alpha}(0)\hat{R}_{0j,\alpha}(0)\langle v'(\tilde{R}_{0i}(t))v'(\tilde{R}_{0j}(s))\rangle_\xi\rangle_{\text{init}} \\
&= \langle \sum_{i,j}\hat{R}_{0i,\alpha}\hat{R}_{0j,\alpha}\langle v'(\tilde{R}_{0i}(t))v'(\tilde{R}_{0j}(s))\rangle_\xi^c\rangle_{\text{init}} \\
&+ \langle \sum_{i,j}\hat{R}_{0i,\alpha}\hat{R}_{0j,\alpha}\langle v'(\tilde{R}_{0i}(t))\rangle_\xi\langle v'(\tilde{R}_{0j}(s))\rangle_\xi\rangle_{\text{init}}
\end{aligned} \tag{94}$$

where we have introduced $\langle\cdot\rangle_0 = \langle\langle\cdot\rangle_\xi\rangle_{\text{init}}$, with $\langle\cdot\rangle_\xi$ the average over thermal noises conditioned on initial conditions $\boldsymbol{R}_{0i}(0), \boldsymbol{R}_{0j}(0)$, and $\langle\cdot\rangle_{\text{init}}$ the full average over initial conditions. In the last two lines of Eq.94, we omit "(0)" for shortening notations and $\langle\cdot\rangle_\xi^c$ stands for the connected correlation.

*Neglecting off-diagonal terms* – We first discuss the connected correlation and focus on an individual correlation term specified by $i, j$ in Eq.94. Recall that (see Eq.6 of the main text) $\tilde{R}_{0i} \approx R_{0i}(0) + \tilde{y}_{0i} + \Delta_u(t)/2R_{0i}(0)$, with $\tilde{y}_{0i} = \hat{\boldsymbol{R}}_{0i}(0)\cdot(\tilde{\boldsymbol{u}}_{0,\alpha}^\perp - \tilde{\boldsymbol{u}}_i)$. The correlation $\langle v'(\tilde{R}_{0i}(t))v'(\tilde{R}_{0j}(s))\rangle_\xi^c$ originates from the correlation $\langle \tilde{y}_{0i}(t)\tilde{y}_{0j}(s)\rangle_\xi^c$. For convenience, we use re-scaled quantities $\bar{y}_i \equiv \tilde{y}_{0i}d$ and $\bar{v}(\bar{y}) \equiv v(d(\tilde{R}-1))$, which are order one. Then

$$\langle v'(\tilde{R}_{0i}(t))v'(\tilde{R}_{0j}(s))\rangle_\xi = d^2\langle \bar{v}'(\bar{y}_i(t))\bar{v}'(\bar{y}_j(s))\rangle_\xi \tag{95}$$

Since both $\bar{v}$ and $\bar{y}$ are order one, it is reasonable to assume

$$\mathcal{O}\left(\langle \bar{v}'(\bar{y}_i(t))\bar{v}'(\bar{y}_j(s))\rangle_\xi^c\right) = \mathcal{O}\left(\langle \bar{y}_i(t)\bar{y}_j(s)\rangle_\xi^c\right) \tag{96}$$

From Eq.82, we obtain the dynamics of $\bar{y}_i$ and $\bar{y}_j$

$$\begin{aligned}
\bar{\zeta}\dot{\bar{y}}_i &= \eta_i + f_i - 2\bar{v}'(\bar{y}_i) + (\hat{R}_{0i,\alpha})^2\bar{v}'(\bar{y}_i) - \sum_{\beta(\neq\alpha)}^{d}\hat{R}_{0i,\beta}\hat{R}_{0j,\beta}\bar{v}'(\bar{y}_j), \\
\bar{\zeta}\dot{\bar{y}}_j &= \eta_j + f_j - 2\bar{v}'(\bar{y}_j) + (\hat{R}_{0j,\alpha})^2\bar{v}'(\bar{y}_j) - \sum_{\beta(\neq\alpha)}^{d}\hat{R}_{0i,\beta}\hat{R}_{0j,\beta}\bar{v}'(\bar{y}_i),
\end{aligned} \tag{97}$$

where $\bar{\zeta} \equiv \zeta/d^2 \sim 1$ and

$$\begin{aligned}
\eta_i &= d^{-1}\hat{\boldsymbol{R}}_{0i}(0)\cdot(\boldsymbol{\xi}_i - \sum_{k\neq 0}\boldsymbol{\nabla} v(\tilde{\boldsymbol{R}}_{ik}) \\
\eta_j &= d^{-1}\hat{\boldsymbol{R}}_{0j}(0)\cdot(\boldsymbol{\xi}_j - \sum_{k\neq 0}\boldsymbol{\nabla} v(\tilde{\boldsymbol{R}}_{jk}) \\
f_i &= d^{-1}\hat{\boldsymbol{R}}_{0i}(0)\cdot(\boldsymbol{\xi}_{0,\alpha}^\perp - \sum_{k\neq i,j}\boldsymbol{\nabla}_\alpha^\perp v(\tilde{\boldsymbol{R}}_{0k})) \\
f_j &= d^{-1}\hat{\boldsymbol{R}}_{0j}(0)\cdot(\boldsymbol{\xi}_{0,\alpha}^\perp - \sum_{k\neq i,j}\boldsymbol{\nabla}_\alpha^\perp v(\tilde{\boldsymbol{R}}_{0k}))
\end{aligned} \tag{98}$$

All terms on r.h.s of Eq.97 are deterministic in $\bar{y}$ except $\eta$ and $f$. Firstly we notice that $\eta_i$ and $\eta_j$ are uncorrelated in the $d\to\infty$ limit for two reasons: (i) according to the Sec.III, degrees of freedom involved in $\eta_i$ are decoupled from those involved in $\eta_j$; (ii) besides the perturbation on $\eta_i$ due to the presence/absence of particle $i$ is negligible and same for $\eta_j$. As a consequence $\eta_i$ and $\eta_j$ can viewed as two independent random forces. Thus the correlation between $\bar{y}_i$ and $\bar{y}_j$, if any, originates from the correlation between $f_i$ and $f_j$. We have $\mathcal{O}(f_if_j) \sim d^{-2}\sum_{\mu\neq\alpha}^d\sum_{\nu\neq\alpha}^d\hat{R}_{0i,\mu}\hat{R}_{0j,\nu}(\xi_{0,\mu} - \sum_k\nabla_\mu v)(\xi_{0,\nu} - \sum_{k'}\nabla_\nu v)$. By self-consistency, it is straightforward to obtain the connected correlations:

$$\langle f_if_j\rangle_\xi^c \sim \begin{cases} 1, & \text{if } i=j \\ d^{-1/2}, & \text{if } i\neq j \end{cases} \tag{99}$$

The last two terms in each of Eq.97 can seen as perturbations since $(\hat{R}_{0i,\alpha})^2 \sim d^{-1}$ and $\sum_{\beta\neq\alpha}\hat{R}_{0i,\beta}\hat{R}_{0j,\beta} \sim d^{-1/2}$ while all other terms are order one. Let $\bar{y}_i^o$ denote the solution of Eq.97 when the perturbations are absent.

Then we have

$$\mathcal{O}\left(\langle \bar{y}_i^o(t)\bar{y}_j^o(s)\rangle_\xi^c\right) = \mathcal{O}\left(\langle f_i(t)f_j(s)\rangle_\xi^c\right) \sim \begin{cases} 1, & \text{if } i=j \\ d^{-1/2}, & \text{if } i\neq j \end{cases} \tag{100}$$

Using linear expansion, the solution of Eq.97 are

$$\begin{aligned} \bar{y}_i(t) \approx& \ \bar{y}_i^o(t) + (\hat{R}_{0i,\alpha})^2 \int_0^t dt' e^{-2\int_{t'}^t \bar{v}''(\bar{y}_i^o(s))ds}\bar{v}'(\bar{y}_i^o(t')) \\ &- \left(\sum_{\beta(\neq\alpha)} \hat{R}_{0i,\beta}\hat{R}_{0j,\beta}\right)\int_0^t dt' e^{-2\int_{t'}^t \bar{v}''(\bar{y}_i^o(s))ds}\bar{v}'(\bar{y}_j^o(t')) \\ \bar{y}_j(t) \approx& \ \bar{y}_j^o(t) + (\hat{R}_{0j,\alpha})^2 \int_0^t dt' e^{-2\int_{t'}^t \bar{v}''(\bar{y}_j^o(s))ds}\bar{v}'(\bar{y}_j^o(t')) \\ &- \left(\sum_{\beta(\neq\alpha)} \hat{R}_{0i,\beta}\hat{R}_{0j,\beta}\right)\int_0^t dt' e^{-2\int_{t'}^t \bar{v}''(\bar{y}_j^o(s))ds}\bar{v}'(\bar{y}_i^o(t')) \end{aligned} \tag{101}$$

For the auto-correlation, it is clear that

$$\begin{aligned} \mathcal{O}\left(\langle \bar{y}_i(t)\bar{y}_i(s)\rangle_\xi^c\right) =& \ \mathcal{O}\left(\langle \bar{y}_i^o(t)\bar{y}_i^o(s)\rangle_\xi^c\right) \\ =& \ \mathcal{O}\left(\langle f_i(t)f_i(s)\rangle_\xi^c\right) = 1 \end{aligned} \tag{102}$$

which with Eq.96 implies that the diagonal contribution of the connected correlation in Eq.94 scales as

$$\begin{aligned} &\langle \sum_i^{\sim d} (\hat{R}_{0i,\alpha})^2 d^2 \langle \bar{v}'(\bar{y}_i(t))\bar{v}'(\bar{y}_i(s))\rangle_\xi^c\rangle_{\text{init}} \\ &\sim d^2 \langle \sum_i^{\sim d} (\hat{R}_{0i,\alpha})^2 \langle \bar{y}_i(t)\bar{y}_i(s)\rangle_\xi^c\rangle_{\text{init}} \\ &\sim d^{2+1-1/2-1/2} \sim d^2 \end{aligned} \tag{103}$$

From Eq.101, the correlation for $i \neq j$ is estimated as

$$\begin{aligned} \mathcal{O}\left(\langle \bar{y}_i\bar{y}_j\rangle_\xi^c\right) =& \ \mathcal{O}\left(\langle \bar{y}_i^o\bar{y}_j^o\rangle_\xi^c\right) \\ &+ \left[(\hat{R}_{0i,\alpha})^2 + (\hat{R}_{0j,\alpha})^2\right]\mathcal{O}\left(\langle \bar{y}_i^o\bar{y}_j^o\rangle_\xi^c\right) \\ &-2\left[\sum_{\beta(\neq\alpha)} \hat{R}_{0i,\beta}\hat{R}_{0j,\beta}\right]\mathcal{O}\left(\langle \bar{y}_i^o\bar{y}_i^o\rangle_\xi^c\right) \end{aligned} \tag{104}$$

Thus the off-diagonal contribution to the connected correlation in Eq.94 is estimated as

$$\begin{aligned} &\mathcal{O}\left(d^2\langle \sum_{i\neq j}^{\sim d^2} \hat{R}_{0i,\alpha}\hat{R}_{0j,\alpha}\langle \bar{v}'(\bar{y}_i)\bar{v}'(\bar{y}_j)\rangle_\xi^c\rangle_{\text{init}}\right) \\ &= \mathcal{O}\left(d^2\langle \sum_{i\neq j}^{\sim d^2} \hat{R}_{0i,\alpha}\hat{R}_{0j,\alpha}\langle \bar{y}_i^o\bar{y}_j^o\rangle_\xi^c\rangle_{\text{init}}\right) \\ &+\mathcal{O}\left(d^2\langle \sum_{i\neq j}^{\sim d^2} \hat{R}_{0i,\alpha}(\hat{R}_{0j,\alpha})^3\langle \bar{y}_i^o\bar{y}_j^o\rangle_\xi^c\rangle_{\text{init}}\right) \\ &+\mathcal{O}\left(d^2\langle \sum_{i\neq j}^{\sim d^2} (\hat{R}_{0i,\alpha})^3\hat{R}_{0j,\alpha}\langle \bar{y}_i^o\bar{y}_j^o\rangle_\xi^c\rangle_{\text{init}}\right) \\ &-\mathcal{O}\left(2d^2\langle \sum_{i\neq j}^{\sim d^2} \hat{R}_{0i,\alpha}\hat{R}_{0j,\alpha}\sum_{\beta(\neq\alpha)}^{d} \hat{R}_{0i,\beta}\hat{R}_{0j,\beta}\rangle_{\text{init}}\right) \\ &= d^{2+1-1/2-1/2-1/2} \\ &+2d^{2+1-1/2-3/2-1/2} \\ &-2d^{2+1-1/2-1/2+(1/2-1/2-1/2)} \\ &= d^{3/2} \end{aligned} \tag{105}$$

We conclude with Eq.105 and Eq.103 that the off-diagonal contribution on the connected correlation of Eq.94 is sub-leading and thus negligible.

We now study the very last term in the force-froce correlation Eq.94. The diagonal contribution is negligible as easily estimated:

$$d^2\langle \sum_i^{\sim d} (\hat{R}_{0i,\alpha})^2 \langle \bar{v}'\rangle_\xi \langle \bar{v}'\rangle_\xi\rangle_{\text{init}} \sim d^{2+1-2/2} \sim d^2 \tag{106}$$

To study the off-diagonal contribution, we use the fact that the $\alpha$ direction is non-special in the initial condition, thus we can write

$$\hat{R}_{0i,\alpha}\hat{R}_{0j,\alpha} = \frac{1}{d}\hat{\boldsymbol{R}}_{0i}\cdot\hat{\boldsymbol{R}}_{0j} \tag{107}$$

and we estimate the upper bound by letting $t = s = 0$ to get

$$\begin{aligned} &\mathcal{O}\left(\langle \sum_{i\neq j}^{\sim d^2} \hat{R}_{0i,\alpha}\hat{R}_{0j,\alpha}\langle v'(t)\rangle_\xi\langle v'(s)\rangle_\xi\rangle_{\text{init}}\right) \\ &\leq \mathcal{O}\left(\sum_{i\neq j}^{\sim d} d^{-1}\langle \hat{\boldsymbol{R}}_{0i}\cdot\hat{\boldsymbol{R}}_{0j} v'(R_{0i})v'(R_{0j})\rangle_{\text{init}}\right) \\ &\leq \mathcal{O}\left(\sum_{i\neq j}^{\sim d} d\langle \hat{\boldsymbol{R}}_{0i}\cdot\hat{\boldsymbol{R}}_{0j}\rangle_{\text{init}}\right) \end{aligned} \tag{108}$$

where $v' \sim d$ is used in the last passage. We may use the average within a sample of typical configuration to evaluate the ensemble average $\langle\cdot\rangle_{\text{init}}$. That is for each pair $i \neq j$ we may write

$$\langle \hat{\boldsymbol{R}}_{0i}\cdot\hat{\boldsymbol{R}}_{0j}\rangle_{\text{init}} \approx \frac{1}{d^2}\sum_{k\neq l} \hat{\boldsymbol{R}}_{0k}\cdot\hat{\boldsymbol{R}}_{0l} \tag{109}$$

For a given $\hat{\boldsymbol{R}}_{0k}$, by isotropy, there are equal number of $\hat{\boldsymbol{R}}_{0l}$ such that $\hat{\boldsymbol{R}}_{0k}\cdot\hat{\boldsymbol{R}}_{0l}\in[a-\delta a,a+\delta a]$ For given $\hat{\boldsymbol{R}}_{0k}$, by isotropy, there must be equal number of $\hat{\boldsymbol{R}}_{0l}$ which give $\hat{\boldsymbol{R}}_{0k}\cdot\hat{\boldsymbol{R}}_{0l}\in[a-\delta a,a+\delta a]$ and those which give $\hat{\boldsymbol{R}}_{0k}\cdot\hat{\boldsymbol{R}}_{0l}\in[-a-\delta a,-a+\delta a]$ with $|a|<1$. Exceptions only take place when $|a|\to 1$, because $k\neq l$ implies $\hat{\boldsymbol{R}}_{0k}\cdot\hat{\boldsymbol{R}}_{0l}\neq 1$, while we still can have $\hat{\boldsymbol{R}}_{0k}\cdot\hat{\boldsymbol{R}}_{0l}\approx -1$ with a probability that scales roughly as $1/S_{d-1}$ where $S_{d-1}\sim\exp(d-1)$ is the area of the $d-1$ unit sphere. By Eq.108, the off-diagonal contribution to the very last term in Eq.94 is negligible. To conclude, the force-force correlation of Eq.94 is dominated by the diagonal contribution when $d\to\infty$

$$\langle\mathcal{F}^{\alpha}_{\alpha}(t)\mathcal{F}^{\alpha}_{\alpha}(s)\rangle_0 \overset{d\to\infty}{=} \sum_{j>0}\langle\nabla_\alpha v(\tilde{\boldsymbol{R}}_{0j}(t))\nabla_\alpha v(\tilde{\boldsymbol{R}}_{0j}(s))\rangle_0 \tag{110}$$

*Restoring the true trajectories in diagonal terms* – Next, we want to compare the diagonal contribution to the force-force correlation in the un-blocked system, i.e.

$$\sum_{j>0}\langle\nabla_\alpha v(\boldsymbol{R}_{0j}(t))\nabla_\alpha v(\boldsymbol{R}_{0j}(s))\rangle,$$
$$\text{where } \boldsymbol{R}_{0j}(t)=\tilde{\boldsymbol{R}}_{0j}(t)-\delta\boldsymbol{u}_j+\delta\boldsymbol{u}^{\perp}_{0,\alpha}+\boldsymbol{u}_{0,\alpha} \tag{111}$$

with Eq.110. In the $d\to\infty$ limit, we already now that

$$\begin{aligned}&\nabla_\alpha v(\boldsymbol{R}_{0j}(t))\nabla_\alpha v(\boldsymbol{R}_{0j}(s))\\ &\qquad\approx\left(\hat{R}_{0j,\alpha}(0)\right)^2 v'(R_{0j}(t))v'(R_{0j}(s))\end{aligned} \tag{112}$$

Next one needs to investigate the difference $R_{0j}(t)-\tilde{R}_{0j}(t)$ due to corrections $\delta\boldsymbol{u}_j$, $\delta\boldsymbol{u}^{\perp}_{0,\alpha}$ and $\boldsymbol{u}_{0,\alpha}$. Up to the leading order correction, we can write

$$\begin{aligned}R_{0j}(t)&\approx\tilde{R}_{0j}(t)+\delta y_j\\ \delta y_j&\hat{=}\hat{\boldsymbol{R}}_{0j}(0)\cdot(\delta\boldsymbol{u}^{\perp}_{0,\alpha}+\boldsymbol{u}_{0,\alpha})\sim d^{-3/2}.\end{aligned} \tag{113}$$

Plugging into Eq.112 and expanding in $\delta y_i$, we arrive at

$$\begin{aligned}&\nabla_\alpha v(\boldsymbol{R}_{0j}(t))\nabla_\alpha v(\boldsymbol{R}_{0j}(s))\\ &\approx\nabla_\alpha v(\tilde{\boldsymbol{R}}_{0j}(t))\nabla_\alpha v(\tilde{\boldsymbol{R}}_{0j}(s))\\ &+\sum_{m\geq1}\frac{1}{m!}\langle\left(\hat{R}_{0j,\alpha}\right)^2 v^{(1+m)}_{0j}(t)\delta y^m_j(t)v'(\tilde{R}_{0j}(s))\rangle_0\\ &+\sum_{n\geq1}\frac{1}{n!}\langle\left(\hat{R}_{0j,\alpha}\right)^2 v'(\tilde{R}_{0j}(t))v^{(1+n)}_{0j}(s)\delta y^n_j(s)\rangle_0\\ &+\sum_{m\geq1,n\geq1}\frac{1}{m!n!}\langle\left(\hat{R}_{0j,\alpha}\right)^2 v^{(1+m)}_{0j}(t)v^{(1+n)}_{0j}(s)\delta y^m_j(t)y^n_j(s)\rangle_0,\end{aligned} \tag{114}$$

where $v^{(1+m)}_{0j}(t)\equiv v^{(1+m)}(\tilde{R}_{0j}(t))$ from which we recognize that the largest correction (when $m=1$ or $n=1$) is of order $d^{1/2}$. Then summing over $\sum^{\sim d}_{j>0}$ results in a total difference of order $d^{3/2}$ of Eq.111 when compared with Eq.110. We thus conclude

$$\begin{aligned}\langle\tilde{F}^{\alpha}_{\alpha}(t)\tilde{F}^{\alpha}_{\alpha}(s)\rangle_0 &\overset{d\to\infty}{=}\sum_{j>0}\langle\nabla_\alpha v(\boldsymbol{R}_{0j}(t))\nabla_\alpha v(\boldsymbol{R}_{0j}(s))\rangle\\ &=\frac{1}{d}\sum_j\langle v(R_{0j}(t))v(R_{0j}(s))\rangle\\ &=\frac{1}{dN}\sum_{i,j,i\neq j}\langle v(R_{ij}(t))v(R_{ij}(s))\rangle\end{aligned} \tag{115}$$

where the last passage relies on the fact that all pair of particles are equivalent.

## XI. CAVITY – TWO PARTICLES PROCESS

To solve for the memory kernel, we need the mean field effective process of the distance between two particles, say the two particles labelled 0 and 1. Recall the distance can be written $R_{01}=R_o+\hat{\boldsymbol{R}}_o\cdot(\boldsymbol{u}_0-\boldsymbol{u}_1)+\Delta/R_o+o(d^{-1})$, where $\Delta=\frac{1}{2}(\boldsymbol{u}_0-\boldsymbol{u}_1)^2=\frac{1}{2}(\boldsymbol{u}_0^2+\boldsymbol{u}_1^2)+\boldsymbol{u}_0\cdot\boldsymbol{u}_1$ and we used $\boldsymbol{R}_o$ for $\boldsymbol{R}_{01}(0)$ for convenience. As $\boldsymbol{u}^2$ concentrates on its average and $\boldsymbol{u}_0\cdot\boldsymbol{u}_1\sim d^{-3/2}$ is sub-leading, we have $\Delta=\langle\boldsymbol{u}^2\rangle$ representing a typical one particle mean squared displacement, which will be solved self-consistently. Then the remaining task is to find out the effective process for $w\hat{=}u_{0,\gamma}-u_{1,\gamma}\hat{=}\hat{\boldsymbol{e}}_\gamma\cdot\boldsymbol{u}_0-\hat{\boldsymbol{e}}_\gamma\cdot\boldsymbol{u}_1$, if we now identify $\hat{\boldsymbol{e}}_\gamma=\hat{\boldsymbol{R}}_o$.

The mean-field limit $d\to\infty$ implies that the typical distance between two neighboring particles of particle 0, say $R_{1j}$ for particle 1 and $j(>1)$, is far beyond the interaction range (knowing that at long range $v(r)\sim r^{-d-\delta}$ with $\delta>0$ for the system to be stable). Thus, the effective random forces $\boldsymbol{\mathcal{F}}_0$ and $\boldsymbol{\mathcal{F}}_1$ are not correlated, as the effective neighbors of particle 0 and those of particle 1 are effectively out of the interaction range. When considering the effective dynamics of $w$, we can copy Eq.92 for $u_{0,\gamma}$ and $u_{1,\gamma}$, but with the exception that now the direction $\hat{\boldsymbol{e}}_\gamma$ is not arbitrarily chosen, but is $\hat{\boldsymbol{e}}_\gamma=\hat{\boldsymbol{R}}_{01}(0)$. In this direction the force $\boldsymbol{\nabla}v(\boldsymbol{R}_{01})$ must be retained as its projection on $\hat{\boldsymbol{e}}_\gamma$ alone is already significant, i.e. $\hat{\boldsymbol{e}}_\gamma\cdot\boldsymbol{\nabla}v(\boldsymbol{R}_{01})\overset{d\to\infty}{=}v'(R_{01})\sim d$. As a result, we have the dynamics for $u_{0,\gamma}$ and $u_{1,\gamma}$

$$\begin{aligned}\zeta\dot{u}_{0,\gamma}&=\xi_{0,\gamma}+\mathcal{F}_{0,\gamma}-\beta\int_0^t ds\mathcal{M}(t-s)\dot{u}_{0,\gamma}(s)-v'(R_{01}),\\ \zeta\dot{u}_{1,\gamma}&=\xi_{1,\gamma}+\mathcal{F}_{1,\gamma}-\beta\int_0^t ds\mathcal{M}(t-s)\dot{u}_{1,\gamma}(s)+v'(R_{01}).\end{aligned} \tag{116}$$

Taking the difference, we find the effective process for $w$:

$$\begin{aligned}\zeta\dot{w}=&-2v'(R_o+w+\Delta/R_o)\\ &+\xi_w+\mathcal{F}_w-\beta\int_0^t ds\mathcal{M}(t-s)\dot{w}(s),\end{aligned} \tag{117}$$

with zero mean Gaussian noises such that

$$\begin{aligned}\langle\xi_w(t)\xi_w(s)\rangle_{\xi_w}&=4T\zeta\delta(t-s),\\ \langle\mathcal{F}_w(t)\mathcal{F}_w(s)\rangle_{\mathcal{F}_w}&=2\mathcal{M}(t-s).\end{aligned} \tag{118}$$

The mean square displacement is formally given by Eq.92 through

$$\Delta(\tau) = d\langle u_{0,\alpha}^2(\tau)\rangle_{\xi,\mathcal{F}} \tag{119}$$

According to Eq.115, the solution is self-consistently given by

$$\begin{aligned}\mathcal{M}(\tau) &= \langle\langle v'(R_o)v'(R_o + w(\tau) + \Delta/R_o)\rangle_{\xi_w,\mathcal{F}_w}\rangle_{R_o} \\ &\hat{=} \frac{1}{d}\int d\boldsymbol{R}_o \langle \frac{1}{N}\sum_{i\neq j}\delta(\boldsymbol{R}_o - \boldsymbol{R}_i + \boldsymbol{R}_j)\rangle_{\text{init}} \\ &\quad\times\langle v'(R_o)v'(R_o + w(\tau) + \Delta/R_o)\rangle_{\xi_w,\mathcal{F}_w} \\ &= \frac{\rho}{d}\int d\boldsymbol{R}_o g(R_o)\langle v'(R_o)v'(R_o + w(\tau) + \Delta/R_o)\rangle_{\xi_w,\mathcal{F}_w}\end{aligned} \tag{120}$$

where $\langle\cdot\rangle_{R_o}$ stands for the average over equilibrium initial configurations and the radial distribution function $g(r) = e^{-\beta v(r)}$ in the large dimension limit [8–10].

## XII. FINAL SET OF EQUATIONS

For solving the liquid dynamics in the mean-field limit $d \to \infty$ where all happen on a length scale of $1/d$, we need to bring the physics back to a scale of order one. For this purpose, we rewrite Eq.117 and the self-consistent condition Eq.120 in terms of the gap variable $h = d(R/\ell - 1)$ where $\ell \equiv 1$ and correspondingly rescale all quantities to order one. The following calculations are in line with one section 5.1.2 of reference [11] up to a factor 2. We define

$$\bar{\zeta}\hat{=}\zeta/d^2, \quad \bar{m}\hat{=}m/d^2, \quad \bar{\xi}_w\hat{=}\xi_w/d, \quad \bar{\mathcal{F}}_w\hat{=}\mathcal{F}/d \tag{121}$$

Note that $v'(R) = d\bar{v}'(h)$, thus we define

$$\bar{\mathcal{M}}(\tau)\hat{=}\mathcal{M}(\tau)/d^2 = \langle\langle \bar{v}'(h_o)\bar{v}'(h(\tau))\rangle_{\bar{\xi}_w,\bar{\mathcal{F}}_w}\rangle_{h_o} \tag{122}$$

where $h_o = d(R_o - 1)$. We then have

$$\begin{aligned}&h(\tau) = h_o + w(\tau)d + \bar{\Delta}(\tau) + \mathcal{O}(d^{-1}) \\ &\bar{\Delta}(\tau)\hat{=}\Delta(\tau)d = \langle(\bar{u}(\tau))^2\rangle_{\bar{\mathcal{F}}_w} \\ &\bar{u}(\tau)\hat{=}du_{0,\alpha}(\tau)\end{aligned} \tag{123}$$

In case where we take into account inertia, the one particle dynamics, e.g. Eq.92 along one arbitrary component is recapped as

$$\bar{m}\ddot{\bar{u}} + \bar{\zeta}\dot{\bar{u}} = \bar{\xi} + \bar{\mathcal{F}} - \beta\int_0^t ds\bar{\mathcal{M}}(t-s)\dot{\bar{u}}(s) \tag{124}$$

with $\bar{\xi}$ and $\bar{\mathcal{F}}$ Gaussian noises satisfying

$$\begin{aligned}&\langle\bar{\xi}(t)\bar{\xi}(s)\rangle_{\bar{\xi}} = 2\bar{\zeta}T\delta(t-s) \\ &\langle\bar{\mathcal{F}}(t)\bar{\mathcal{F}}(s)\rangle_{\bar{\mathcal{F}}} = \bar{\mathcal{M}}(t-s)\end{aligned} \tag{125}$$

The two particle process Eq.117 now reads

$$\begin{aligned}\bar{m}\ddot{h} + \bar{\zeta}\dot{h} &= \mathcal{B}(t) - 2\bar{v}'(h) + \sqrt{2}\bar{\xi} + \sqrt{2}\bar{\mathcal{F}} \\ &\quad -\beta\int_0^t ds\bar{\mathcal{M}}(t-s)\dot{h}(s) \\ \mathcal{B}(t)&\hat{=}\bar{m}\ddot{\bar{\Delta}}(t) + \bar{\zeta}\dot{\bar{\Delta}}(t) + \beta\int_0^t ds\bar{\mathcal{M}}(t-s)\dot{\bar{\Delta}}(s)\end{aligned} \tag{126}$$

where the mean square displacement can be formally computed using Eq.124:

$$\bar{\Delta}(t) = \langle(\bar{u}(t))^2\rangle_{\bar{\xi},\bar{\mathcal{F}}} \tag{127}$$

which after a lengthy calculation [11] reduces to the temperature, i.e. $\mathcal{B}(t) = 2T$, in the equilibrium case. Finally taking profit from the isotropy of the integral in Eq.120 by working with with polar coordinate, we rewrite the self-consistent condition

$$\begin{aligned}\bar{\mathcal{M}}(\tau) &= \frac{\rho}{d}\int \Omega_d R_o^{d-1}dR_o e^{-\beta\bar{v}(h_o)}\langle\bar{v}'(h_o)\bar{v}'(h(\tau))\rangle_{\bar{\xi},\bar{\mathcal{F}}} \\ &= \frac{\rho}{d^2}\int \Omega_d(1+\frac{h_o}{d})^{d-1}dh_o e^{-\beta\bar{v}(h_o)}\langle\bar{v}'(h_o)\bar{v}'(h(\tau))\rangle_{\bar{\xi},\bar{\mathcal{F}}} \\ &= \hat{\varphi}\int dh_o e^{h_o-\beta\bar{v}(h_o)}\langle\bar{v}'(h_o)\bar{v}'(h(\tau))\rangle_{\bar{\xi},\bar{\mathcal{F}}}\end{aligned} \tag{128}$$

where $\Omega_d$ the solid angle and $\hat{\varphi} = \frac{\rho\Omega_d}{d^2}$ the rescaled packing fraction if the interaction range $\ell \equiv 1$ is considered roughly as the diameter of particles.

## XIII. RANDOM LORENTZ GAS

The random Lorentz gas (RGL) problem can be defined as following. Take at random a configuration of particle positions $\{\boldsymbol{R}_0, \{\boldsymbol{R}_j\}_{j>0}\}$ from the equilibrium Boltzmann distribution as defined by $\propto \exp\left(-\beta\left[\sum_{k>i\geq 0} v(\boldsymbol{R}_i - \boldsymbol{R}_k)\right]\right)$, then fix particle positions $\boldsymbol{R}_{j>0}$ and let only particle $\boldsymbol{R}_0$ move according to the following dynamics

$$\zeta\dot{\boldsymbol{R}}_0 = \boldsymbol{\xi}_0 - \sum_{j>0}\boldsymbol{\nabla}v(\boldsymbol{R}_0 - \boldsymbol{R}_j). \tag{129}$$

The dynamics of the random Lorentz gas can be viewed as a specific case of the standard $N \to \infty$ particle problem where the particle zero $\boldsymbol{R}_0$ moves as in Eq.129 and particles $\boldsymbol{R}_{j>0}$ follow

$$\zeta^*\dot{\boldsymbol{R}}_j = \boldsymbol{\xi}_j - \sum_{i\neq 0}\boldsymbol{\nabla}v(\boldsymbol{R}_j - \boldsymbol{R}_i), \tag{130}$$

within the limit $\zeta/\zeta^* \to 0$. Using a simple diffusion argument, one concludes

$$\frac{(\boldsymbol{R}_j(t) - \boldsymbol{R}_j(0))^2}{(\boldsymbol{R}_0(t) - \boldsymbol{R}_0(0))^2} \sim \frac{\zeta}{\zeta^*} \to 0, \tag{131}$$

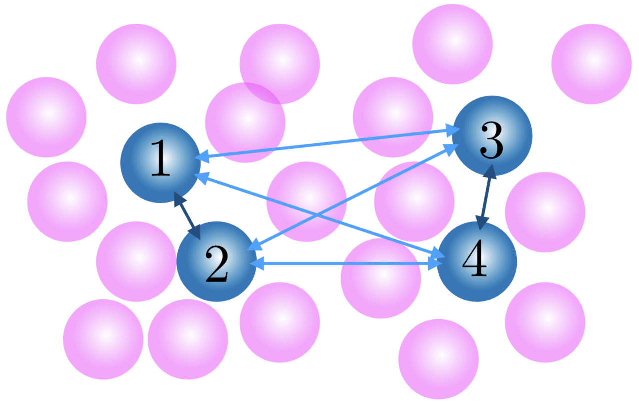


FIG. 1. Illustration of the real-space meaning of liquid-state cluster dynamical mean-field theory.

i.e. the particles $j > 0$ are immobile compared with particle zero. In addition, since we keep the same interaction potential, the equilibrium measure of the configuration of particle positions remains the same.

This situation allows us to apply our method for deriving the mean-field theory of the RLG problem. We only need to accommodate the previous results of standard DMFT according to the limit $\zeta/\zeta^* \to 0$ to obtain the correct equations. For the one particle (particle $\boldsymbol{R}_0$) process of the RLG, the exact same calculation applies and leads to the same equation as found in Eq.92 except that $\boldsymbol{u}_j = 0$ in the argument of $\boldsymbol{\mathcal{F}}_0$ for particles $j > 0$, which are immobile.

To solve the memory kernel in the one particle process, we need the two particle process in the limit $\zeta/\zeta^* \to 0$, for which we may multiply $\zeta/\zeta^*$ on both sides of the second line of Eq.116 and take the difference to obtain the dynamics of $\zeta\frac{d}{dt}(\boldsymbol{R}_0 - \boldsymbol{R}_1)$. Because of the multiplication by $\zeta/\zeta^*$ of all members of the second equation of Eq.116, all forces coming from the second line of Eq.116 are neglected and so is the motion of particle $j$ inside the bare force term between the two particles. Thus, defining now $w(t)\hat{=}\hat{\boldsymbol{e}}_\gamma \cdot (\boldsymbol{W}(t) - \boldsymbol{W}(0))$ with $\hat{\boldsymbol{e}}_\gamma\hat{=}(\boldsymbol{R}_0(0) - \boldsymbol{R}_j(0))/|\boldsymbol{R}_0(0) - \boldsymbol{R}_j(0)|$, we have

$$\zeta\dot{w} = -v'(R^*_{0j} + w + \frac{\Delta_{\boldsymbol{u}}}{2R^*_{0j}}) \tag{132}$$

$$+ \xi_\gamma + \mathcal{F}_\gamma(t) - \beta\int_0^t ds\langle\mathcal{F}_\gamma(t)\mathcal{F}_\gamma(s)\rangle\dot{w}(s), \tag{133}$$

where $\Delta_{\boldsymbol{u}}(t)\hat{=}\langle\boldsymbol{u}(t)\cdot\boldsymbol{u}(t)\rangle = \langle(\boldsymbol{R}_0(t) - \boldsymbol{R}_0(0))^2\rangle$ is the mean square displacement which can be expressed by the one particle process of the RLG.

## XIV. SKETCH OF CLUSTER DMFT

In order to study the slow dynamics of supercooled liquids in low spatial dimensions, we sketch the construction of a cluster DMFT (cDMFT) here, inspired by work in the study of correlated quantum systems. [12, 13] The sharp dynamical transition found in the DMFT[14, 15] is smeared out in low dimensional supercooled liquids, a fact attributable to collective motion of particles within a spatial range possibly associated to the "point-to-set" length [16–18]. This collective motion is absent in the mean-field theory, as it accounts only for correlations within a pair of particles. To incorporate correlations among several particles and still keep the theory tractable, we consider a cluster (containing several particles), instead of just one particle, embedded in a self-consistent bath composed of other equivalent clusters. This idea is sketched in Fig.1. By analogy with DMFT, we expect this approach to include a subset of higher order terms in $1/d$, leading to equations of the form

$$\begin{aligned}\zeta\dot{\boldsymbol{u}}_1 &= \boldsymbol{\xi}_1 + \boldsymbol{\mathcal{F}}_1 - \boldsymbol{\nabla}v(\boldsymbol{R}_{12}) + \boldsymbol{F}^{\rm pmf}(\boldsymbol{R}_{12}) - \beta\int_0^t \mathcal{M}_{\rm self}(\tau)\dot{\boldsymbol{u}}_1(t-\tau)d\tau - \beta\int_0^t \mathcal{M}_{\rm cross}(\tau')\dot{\boldsymbol{u}}_2(t-\tau')d\tau',\\ \zeta\dot{\boldsymbol{u}}_2 &= \boldsymbol{\xi}_2 + \boldsymbol{\mathcal{F}}_2 - \boldsymbol{\nabla}v(\boldsymbol{R}_{21}) + \boldsymbol{F}^{\rm pmf}(\boldsymbol{R}_{21}) - \beta\int_0^t \mathcal{M}_{\rm self}(\tau)\dot{\boldsymbol{u}}_2(t-\tau)d\tau - \beta\int_0^t \mathcal{M}_{\rm cross}(\tau')\dot{\boldsymbol{u}}_1(t-\tau')d\tau',\end{aligned} \tag{134}$$

where $\boldsymbol{F}^{\rm pmf}$ is the potential mean force due to the interaction between the cluster and its environment and the fluctuating forces $\boldsymbol{\mathcal{F}}_1$ and $\boldsymbol{\mathcal{F}}_2$ satisfy

$$\begin{aligned}\langle\mathcal{F}_{1,\mu}(\tau)\otimes\mathcal{F}_{1,\nu}(s)\rangle &= \langle\mathcal{F}_{2,\mu}(\tau)\otimes\mathcal{F}_{2,\nu}(s)\rangle = \delta_{\mu\nu}\mathcal{M}_{\rm self}(\tau - s),\\ \langle\mathcal{F}_{1,\mu}(\tau)\otimes\mathcal{F}_{2,\nu}(s)\rangle &= \langle\mathcal{F}_{2,\mu}(\tau)\otimes\mathcal{F}_{1,\nu}(s)\rangle = \delta_{\mu\nu}\mathcal{M}_{\rm cross}(\tau - s).\end{aligned} \tag{135}$$

Since physically, $\boldsymbol{\mathcal{F}}_1 = -\sum_{j>2}\boldsymbol{\nabla}v(\boldsymbol{R}_{1j})$ and $\boldsymbol{\mathcal{F}}_2 = -\sum_{j>2}\boldsymbol{\nabla}v(\boldsymbol{R}_{2j})$, to solve the memory kernels $\mathcal{M}_{\rm self}$ and

$\mathcal{M}_{\rm cross}$, one needs to write down a two-cluster process dynamics. If a second cluster is composed of particles 3 and 4, the entire set of two-cluster equations is written

$$\begin{aligned}
\zeta\dot{\boldsymbol{u}}_1 &= \boldsymbol{\xi}_1 + \boldsymbol{\mathcal{F}}_1 + \boldsymbol{F}^{\rm pmf}(\boldsymbol{R}_{12}) - \boldsymbol{\nabla} v(\boldsymbol{R}_{12}) - \boldsymbol{\nabla} v(\boldsymbol{R}_{13}) - \boldsymbol{\nabla} v(\boldsymbol{R}_{14}) - \beta\int_0^t \mathcal{M}_{\rm self}(\tau)\dot{\boldsymbol{u}}_1(t-\tau)d\tau - \beta\int_0^t \mathcal{M}_{\rm cross}(\tau')\dot{\boldsymbol{u}}_2(t-\tau')d\tau', \\
\zeta\dot{\boldsymbol{u}}_2 &= \boldsymbol{\xi}_2 + \boldsymbol{\mathcal{F}}_2 + \boldsymbol{F}^{\rm pmf}(\boldsymbol{R}_{21}) - \boldsymbol{\nabla} v(\boldsymbol{R}_{21}) - \boldsymbol{\nabla} v(\boldsymbol{R}_{23}) - \boldsymbol{\nabla} v(\boldsymbol{R}_{24}) - \beta\int_0^t \mathcal{M}_{\rm self}(\tau)\dot{\boldsymbol{u}}_2(t-\tau)d\tau - \beta\int_0^t \mathcal{M}_{\rm cross}(\tau')\dot{\boldsymbol{u}}_1(t-\tau')d\tau', \\
\zeta\dot{\boldsymbol{u}}_3 &= \boldsymbol{\xi}_3 + \boldsymbol{\mathcal{F}}_3 + \boldsymbol{F}^{\rm pmf}(\boldsymbol{R}_{34}) - \boldsymbol{\nabla} v(\boldsymbol{R}_{31}) - \boldsymbol{\nabla} v(\boldsymbol{R}_{32}) - \boldsymbol{\nabla} v(\boldsymbol{R}_{34}) - \beta\int_0^t \mathcal{M}_{\rm self}(\tau)\dot{\boldsymbol{u}}_3(t-\tau)d\tau - \beta\int_0^t \mathcal{M}_{\rm cross}(\tau')\dot{\boldsymbol{u}}_4(t-\tau')d\tau', \\
\zeta\dot{\boldsymbol{u}}_4 &= \boldsymbol{\xi}_4 + \boldsymbol{\mathcal{F}}_4 + \boldsymbol{F}^{\rm pmf}(\boldsymbol{R}_{43}) - \boldsymbol{\nabla} v(\boldsymbol{R}_{41}) - \boldsymbol{\nabla} v(\boldsymbol{R}_{42}) - \boldsymbol{\nabla} v(\boldsymbol{R}_{43}) - \beta\int_0^t \mathcal{M}_{\rm self}(\tau)\dot{\boldsymbol{u}}_4(t-\tau)d\tau - \beta\int_0^t \mathcal{M}_{\rm cross}(\tau')\dot{\boldsymbol{u}}_3(t-\tau')d\tau'.
\end{aligned} \tag{136}$$

From these equations, the memory kernels can be solved self-consistently by computing the correlations among the bare forces among the four particles. A full derivation of these equations and their numerical treatment will be contained in a future publication.


[1] G. Parisi, P. Urbani, and F. Zamponi, *Theory of simple glasses: exact solutions in infinite dimensions* (Cambridge University Press, 2020).

[2] R. Mari, F. Krzakala, and J. Kurchan, Jamming versus glass transitions, Physical review letters **103**, 025701 (2009).

[3] P. Mazur and I. Oppenheim, Molecular theory of brownian motion, Physica **50**, 241 (1970).

[4] J. Deutch and I. Oppenheim, Molecular theory of brownian motion for several particles, Journal of Chemical Physics **54**, 3547 (1971).

[5] T. Hudson and Z. H. Li, Coarse-graining of overdamped langevin dynamics via the mori-zwanzig formalism, Multiscale Modeling & Simulation **18**, 1113 (2020).

[6] D. J. Evans and G. Morriss, *Statistical Mechanics of Nonequilibrium Liquids*, 2nd ed. (Cambridge University Press, 2008).

[7] One can easily check that the terms of $\mathcal{O}(u_{0,\alpha}^2)$ in the expansion give sub-leading contribution compared to the first order terms in Eq.81 and Eq.82. However, if one were to perform the Taylor expansion in terms of the entire vector $\boldsymbol{u}_0$, i.e. making the reference as the system where the tagged particle is fully blocked, one also easily checks that the second order contribution is also order $d$, thus can not be neglected and prevent us from treating the entire vector $\boldsymbol{u}_0$ as a linear perturbation.

[8] H. Frisch, N. Rivier, and D. Wyler, Classical hard-sphere fluid in infinitely many dimensions, Physical review letters **54**, 2061 (1985).

[9] D. Wyler, N. Rivier, and H. Frisch, Hard-sphere fluid in infinite dimensions, Physical Review A **36**, 2422 (1987).

[10] H. Frisch and J. Percus, High dimensionality as an organizing device for classical fluids, Physical Review E **60**, 2942 (1999).

[11] E. Agoritsas, G. Biroli, P. Urbani, and F. Zamponi, Out-of-equilibrium dynamical mean-field equations for the perceptron model, Journal of Physics A: Mathematical and Theoretical **51**, 085002 (2018).

[12] G. Kotliar, S. Y. Savrasov, G. Palsson, and G. Biroli, Cellular dynamical mean field approach to strongly correlated systems, Physical Review Letters **87**, 186401 (2001).

[13] T. A. Maier, M. Jarrell, T. Pruschke, and M. H. Hettler, Quantum cluster theories, Reviews of Modern Physics **77**, 1027 (2005).

[14] T. Maimbourg, J. Kurchan, and F. Zamponi, Solution of the dynamics of liquids in the large-dimensional limit, Physical Review Letters **116**, 015902 (2016).

[15] A. Manacorda, G. Schehr, and F. Zamponi, Numerical solution of the dynamical mean field theory of infinite-dimensional equilibrium liquids, The Journal of chemical physics **152**, 164506 (2020).

[16] J.-P. Bouchaud and G. Biroli, On the adam-gibbs-kirkpatrick-thirumalai-wolynes scenario for the viscosity increase in glasses, Journal of Chemical Physics **121**, 7347 (2004).

[17] T. R. Kirkpatrick, D. Thirumalai, and P. G. Wolynes, Scaling concepts for the dynamics of viscous liquids near an ideal glassy state, Physical Reivew A **40**, 1045 (1989).

[18] L. Berthier, P. Charbonneau, and S. Yaida, Efficient measurement of point-to-set correlations and overlap fluctuations in glass-forming liquids, Journal of Chemical Physics **144**, 024501 (2016).

[19] J. Kurchan, T. Maimbourg, and F. Zamponi, Statics and dynamics of infinite-dimensional liquids and glasses: a parallel and compact derivation, Journal of Statistical Mechanics: Theory and Experiment **2016**, 033210 (2016).

[20] M. Mézard, G. Parisi, and M. A. Virasoro, *Spin glass theory and beyond: An Introduction to the Replica Method and Its Applications*, Vol. 9 (World Scientific Publishing Company, 1987).

[21] E. Agoritsas, T. Maimbourg, and F. Zamponi, Out-of-equilibrium dynamical equations of infinite-dimensional particle systems i. the isotropic case, Journal of Physics A: Mathematical and Theoretical **52**, 144002 (2019).

[22] R. Zwanzig, Nonlinear generalized Langevin equations, Journal of Statistical Physics **9**, 215 (1973).

[23] L. Berthier and G. Biroli, Theoretical perspective on the glass transition and amorphous materials, Reviews of Modern Physics **83**, 587 (2011).

[24] V. Lubchenko and P. G. Wolynes, Theory of structural glasses and supercooled liquids, Annual Review of Physical Chemistry **58**, 235 (2007).

[25] S. Karmakar, C. Dasgupta, and S. Sastry, Length scales in glass-forming liquids and related systems: a review, Reports on Progress in Physics **79**, 016601 (2015).

[26] S. Karmakar, C. Dasgupta, and S. Sastry, Growing length scales and their relation to timescales in glass-forming liquids, Annual Review of Condensed Matter Physics **5**, 255 (2014).

[27] A. Georges, G. Kotliar, W. Krauth, and M. J. Rozenberg, Dynamical mean-field theory of strongly correlated fermion systems and the limit of infinite dimensions, Reviews of Modern Physics **68**, 13 (1996).

[28] A. Ikeda and K. Miyazaki, Mode-coupling theory as a mean-field description of the glass transition, Physical Review Letters **104**, 255704 (2010).

[29] B. Schmid and R. Schilling, Glass transition of hard spheres in high dimensions, Physical Review E **81**, 041502 (2010).

[30] D. R. Reichman and P. Charbonneau, Mode-coupling theory, Journal of Statistical Mechanics-Theory and Experiment (2005).

[31] T. A. de Pirey, G. Lozano, and F. van Wijland, Active hard spheres in infinitely many dimensions, Physical Review Letters **123**, 260602 (2019).

[32] G. Biroli, P. Charbonneau, E. I. Corwin, Y. Hu, H. Ikeda, G. Szamel, and F. Zamponi, Interplay between percolation and glassiness in the random lorentz gas, Physical Review E **103**, L030104 (2021).

[33] R. Mannella and P. V. E. McClintock, Ito versus stratonovich: 30 years later, Fluctuation and Noise Letters **11**, 1240010 (2012).

[34] T. R. Kirkpatrick and P. G. Wolynes, Connections between some kinetic and equilibrium theories of the glass-transition, Physical Review A **35**, 3072 (1987).

[35] W. Götze, *Complex dynamics of glass-forming liquids: A mode-coupling theory*, Vol. 143 (OUP Oxford, 2008).

[36] M. Minsky and S. A. Papert, *Perceptrons: An introduction to computational geometry* (MIT press, 2017).

[37] H. A. Lorentz, *Le mouvement des électrons dans les métaux, Arch. Néerl. 10, 336 (1905); In collected papers*, Vol. 3, p. 180.

[38] G. Szamel, Simple theory for the dynamics of mean-field-like models of glass-forming fluids, Phys. Rev. Lett. **119**, 155502 (2017).
